# Supplementary material for: Deep Coregionalization for the Emulation of Spatial-Temporal Fields
Source: arXiv:1910.07577 source file (2019-10-16)
Supplement: Supplementary file 1 [file appendix_v1.tex]

\section{Appendix}

\begin{lemma}
	A LMC model produces multivariate Gaussian distribution: $\y^{(f)}(\x) = \mathcal{N}(\0, \B^{(f)} \K_r^{(f)}(\x,\x') {\B^{(f)}}^T ) $, where $\K_r^{(f)}(\x,\x') = \diag\left(k^{(f)}_1(\x,\x'),\dots,k^{(f)}_R(\x,\x') \right)$.
	\end{lemma}
\begin{proof}
Following equation.\ref{eq:lmc}, we can easily calculate the mean and covariance of the LMC model as,
\begin{equation}
\begin{aligned}
\EE[\y(\x)] & = \B \EE[\z(\x)] = \0\\
\cov[\y(\x),\y(\x')] & = \EE[\B \z(\x) \z(\x')^T \B^T] - \EE[\B \z(\x)] \EE[\B \z(\x')]^T\\
& = \B \EE [\z(\x) \z(\x)^T] \B^T = \B  \cov[\z(\x)] \B^T. \\ 
\end{aligned}
\end{equation}
The covariance matrix is diagonal, \ie $\cov[\z(\x)]= \diag\left(k^{(f)}_1(\x,\x'), \dots,k^{(f)}_R(\x,\x') \right)$, 
since the LMC requires $z_r(\x)$ to be independent.
\end{proof}
	
\begin{lemma}
	With the LMC representation, the deep kernel always has a equivalent compact kernel function based on previous latent process posterior,
	\[	k^{(f)}\left(\x, \x', \y^{(f-1)}(\x), \y^{(f-1)}(\x')\right) = \hat{k}^{(f)}\left(\x, \x', \z^{(f-1)}(\x), \z^{(f-1)}(\x')\right) \].
	%	If the covariance function is stationary that takes the general form of $k^{(f)}_y(\y(\x), \y(\x')) = h \left( (\y(\x)-\y(\x')) \bSigma^{-1} (\y(\x)-\y(\x'))^T \right) $, there exist a compact kernel of the same form as,
	%	\[
	%	h \left( (\z(\x)-\z(\x')) \widehat{\bSigma}^{-1} (\z(\x)-\z(\x'))^T \right) 
	%	\]
\end{lemma}
\begin{proof}
The compact kernel always exists since $\y^{(f-1)}(\x)$ essentially is linear projection of $\z^{(f-1)}(\x)$ and the degree of freedom is control by $\z^{(f-1)}(\x)$.
\begin{equation}
\begin{aligned}
& k^{(f)}\left(\x, \x', \y^{(f-1)}(\x), \y^{(f-1)}(\x')\right) \\
& = k^{(f)}\left(\x, \x', \B\z^{(f-1)}(\x), \B\z^{(f-1)}(\x')\right) \\
&= \hat{k}^{(f)}\left(\x, \x', \z^{(f-1)}(\x), \z^{(f-1)}(\x)\right).
\end{aligned}
\end{equation}
where $\hat{k}$ is a composite function absorbing $\B$. 
%Depending on the kernel we used, we can end up with a kernel function  

\end{proof}

\begin{prop}
	If each fidelity admits a LMC representation, there exist a low-rank independent deep structure that describes the flow of data and uncertainty,
	\[
	z_r^{(f)}(\x) = \widehat{g}_r^{(f)}(\x, \z_*^{(f-1)}(\x)).
	\]
\end{prop}
\begin{proof}
According to the properties of a LMC, if  
According to the definition of a GP autoregressive model, given input $\x$ and the result of previous fidelity GP $\y^{(f-1)}(\x)$, the next fidelity is a GP and thus is fully described using the mean and covariance. 
following the zero mean assumption, we only need to consider the covariance. 
We can write the covariance function between $i$ and $j$ output as,
$k^{(f)}(i,j,\x,\x',\y^{(f-1)}(\x),\y^{(f-1)}(\x'))$ without assuming any particular structure, such as the separable structure.
\begin{equation}
\begin{aligned}
\cov[y_i^{(f)}(\x),y_j^{(f)}(\x')] 
&= k^{(f)}(i,j,\x,\x',\y^{(f-1)}(\x),\y^{(f-1)}(\x'))\\
\cov[\B_{:i} \z^{(f)}(\x),\B_{:j} \z^{(f)}(\x')] 
&=k^{(f)}(i,j,\x,\x',\B^{(f-1)} \z^{(f-1)}(\x),\B^{(f-1)} \z^{(f-1)}(\x'))\\
\B_{:i} \cov[ \z^{(f)}(\x),\z^{(f)}(\x')] \B_{:j}^T
&=\hat{k}^{(f)}(i,j,\x,\x', \z^{(f-1)}(\x),\z^{(f-1)}(\x'))\\
% \cov[ \z^{(f)}(\x),\z^{(f)}(\x')] 
%&= \B_{:i}^T \hat{k}^{(f)}(i,j,\x,\x', \z^{(f-1)}(\x),\z^{(f-1)}(\x')) \B_{:j}\\
\end{aligned}
\end{equation}

let $[\K]_{ij} = k^{(f)}(i,j,\x,\x',\B^{(f-1)} \z^{(f-1)}(\x),\B^{(f-1)} \z^{(f-1)}(\x')) $ be the covariance matrix computed by the kernel function. Note that there is no particular assumption over the form of the kernel function.
Assuming the high dimensional deep GP structure exist, we have,
\begin{equation}
\begin{aligned}
\cov[y_i^{(f)}(\x),y_j^{(f)}(\x')] 
&= \K \\
\cov[\B \z^{(f)}(\x),\B \z^{(f)}(\x')] 
&=\K\\
\B \cov[ \z^{(f)}(\x),\z^{(f)}(\x')] \B^T
&=\K\\
\cov[ \z^{(f)}(\x),\z^{(f)}(\x')] 
&=\B^T \K \B.
% \cov[ \z^{(f)}(\x),\z^{(f)}(\x')] 
%&= \B_{:i}^T \hat{k}^{(f)}(i,j,\x,\x', \z^{(f-1)}(\x),\z^{(f-1)}(\x')) \B_{:j}\\
\end{aligned}
\end{equation}
This means that unless $\K$ is diagonal, which mean the high dimensional output of

\end{proof}

\subsection{Some proof}
Extending the deep GP multi-variate is non-trivial due to the high dimensional nature.
even when $R$ is of moderate size, Equation\eqref{eq:deep gp} can not direct extend to high dimensional outputs due to the massive inputs passed down from posterior inference of previous fidelity. 
While we can extend Equation\eqref{eq:deep gp} to a standard deep GP that samples multiple functions in each layer, it feeds all the outputs into the next layer and hence is not scalable to a large number of outputs, say, millions. 
Moreover, deep GPs consider the outputs in each layer as independent (given the inputs) and it is unclear how to model the strong output correlations, which is crucial for learning with a small set of training examples. 
%
%To address these problems, we inherit the low rank structure of LMC, \ie a small number of bases and weights,  to handle massive outputs. 
%Based on the low rank structure, we develop a deep model to conduct multi-fidelity learning. Our model can be considered as a variant of the standard deep GP. 
%
%Inspired by the LMC, we assume a low-rank structure for data at each fidelity level as,
%\begin{equation}
%\y^{(F)}(x) = \sum_{f=1}^{F} \B^{(f)} \z^{(f)}(\x), 
%\end{equation} 
%where $\B^{(f)}$ is the bases and $\z^{(f)}(\x)$ is the GP for each fidelity.
%$\z^{(f)}$ is a deep GP such that previous information could be passed to the next fidelity level.
%
%This allow us to model the high dimensional correlation using a low dimensional data flow.
%Following the formulation of \eqref{eq:deep gp}, we have 
%\begin{equation}
%\cov(\y(x),\y(x')) = \B^{(f)} \I {B^{(f)}}^T = k^{(f)}(\x,\x',\y(x),\y(x'))
%\end{equation}
%
%\begin{equation}
%\cov(\z(x),\z(x')) = \I = k^{(f)}(\x,\x',\y(x),\y(x'))
%\end{equation}
%
%\begin{equation}
%k^{(f)} = k_x^{(f)}(\x, \x'; \btheta_{fx} ) \cdot k_y^{(f)}(\y^{(f-1)}(\x), \y^{(f-1)}(\x'); \btheta_{fy} ) +k_{\delta}^{(f)}(\x, \x'; \btheta_{f\delta}),
%\end{equation}
%
Once the bases $\B$ has been learned form the data, the information only flow in the related latent process, thus,
\begin{equation}
\z^{(f)}(\x) = \g^{(f)}(\z^{(f-1)}(\x),\x)
\end{equation}
with 
\begin{equation}
\cov(\z^{(f)}(x),\z^{(f)}(x')) = \I  \otimes k^{(f)}(\z^{(f-1)}(x'),\z^{(f-1)}(x))
\end{equation}

Now we combine the idea LMC to model the high dimensional multi-fidelity data by substituting Equation \eqref{eq:lmc} to Equation \eqref{eq:deep gp}, we have,
\begin{equation}
\label{eq:deep lmc}
{\B^{(f)}} \z^{(f)}(\x) =  \g^{(f)}\left(\x, \B^{(f-1)}\z_*^{(f-1)}(\x)\right),
\end{equation}

Since the covariance is only determined by the latent process $\K_r^{(f)}(\x,\x')$ 

\begin{equation}
k^{(f)}\left(\x, \x', y(\x), y(\x)\right) = k_x^{(f)}(\x, \x'; \btheta_{fx} ) \cdot k_y^{(f)}(y^{(f-1)}(\x), y^{(f-1)}(\x'); \btheta_{fy} ) +k_{\delta}^{(f)}(\x, \x'; \btheta_{f\delta}),
\end{equation}

%Sine the LMC has a tractable form, the exiting framework of univariate deep GPs will remain the same. 
Using the LMC representation, the hyperparameter needed for kernel function $k^{(f)}$ is now proportional to $R$ rather than $d$; the cumbersome covariance could be represented using a more efficient compact form as,
$k^{(f)} = k_x^{(f)}(\x, \x'; \btheta_{fx} ) \cdot k_z^{(f)}(\z^{(f-1)}(\x), \z^{(f-1)}(\x'); \btheta_{fz} ) + k_{\delta}^{(f)}(\x, \x'; \btheta_{f\delta})$, where $\btheta_{fz} \in \RR^R$, $R \ll d$.
\begin{lemma}
	If the covariance function is stationary that takes the general form of $k^{(f)}_y(\y(\x), \y(\x')) = h \left( (\y(\x)-\y(\x')) \bSigma^{-1} (\y(\x)-\y(\x'))^T \right) $, there exist a compact kernel of the same form as,
	\[
	h \left( (\z(\x)-\z(\x')) \widehat{\bSigma}^{-1} (\z(\x)-\z(\x'))^T \right) 
	\]
\end{lemma}
%\begin{proposition}
%Using the LMC representation, the hyperparameter needed for kernel function $k^{(f)}$ is now proportional to $R$ rather than $d$; the cumbersome covariance could be represented using a more efficient compact form as,
%$k^{(f)} = k_x^{(f)}(\x, \x'; \btheta_{fx} ) \cdot k_z^{(f)}(\z^{(f-1)}(\x), \z^{(f-1)}(\x'); \btheta_{fz} ) +k_{\delta}^{(f)}(\x, \x'; \btheta_{f\delta})$, where $\btheta_{fz} \in \RR^R$, $R \ll d$.
%%If the deep kernel for the previous fidelity data is stationary, 
%\end{proposition}
\begin{proof}
	
	This implies that there is a low-rank deep latent structure for the latent process that simplified the high dimensional correlation.  
	This properties is extremely useful since most successful application of deep GP are based on stationary deep kernel, e.g., the ARD kernel, which is a specific case of $\bSigma^{-1}$ being a diagonal matrix and $h(\cdot)$ being an exponential function.

	Assume a stationary kernel that takes a general form as $k(\y(x), \y(x') ) = h(||\y(x) - \y(x')|| )$, we can derive,
	\begin{equation}
	k(\y(x), \y(x') ) = h(||\y(x) - \y(x')|| ) = h\left( ||\B (\z(x) - \z(x')|| \right)
	\end{equation}
	
	$\B$ can be treated as an affine transformation that could be  
	
\end{proof}
This is also true for other type of kernel...
