# Supplementary material for: Deep Coregionalization for the Emulation of Spatial-Temporal Fields
Source: arXiv:1910.07577 source file (2019-10-16)
Supplement: Supplementary file 2 [file appendix_v2.tex]

\begin{appendices}
\section{Proof of Lemma~\ref{LEMMA1} } 
\label{ap:proof_l1}
We provide a proof of Lemma~\ref{LEMMA1} here. 
Firstly, we can write the  full covariance specified by Eq.~\eqref{eq:deep gp kernel2} in a matrix form, 
%For a kernel function having the Eq.\eqref{eq:deep gp kernel2}, we can directly write the covariance of the whole vector $\y^{(f)}(\x)$ as 
\begin{equation}
\label{eq:sepInMatrix}
\begin{aligned}
\cov\left[\y^{(f)}(\x),\y^{(f)}(\x')\right] &= \K_d^{(f)} \cdot k_x^{(f)}(\x,\x') \cdot k_y^{(f)}\left([\x, \y_*^{(f-1)}(\x) ], [\x', \y_*^{(f-1)}(\x') ]\right)\\
 &= \K_d^{(f)} \cdot k_{xy}^{(f)}\left([\x, \y_*^{(f-1)}(\x) ], [\x', \y_*^{(f-1)}(\x') ]\right)
\end{aligned}
\end{equation}
where $[\K^{(f)}_d]_{ij}=k^{(f)}_d(i,j)$ is the covariance matrix of outputs and $k_{xy}^{(f)}$ is a representation of the kernel function depends on $\x$  and $\y_*^{(f-1)}(\x)$. Since a covariance matrix is always p.s.d., $\K^{(f)}_d$ admits an eigendecomposition of 
\begin{equation}
\label{eq:eigen}
\K^{(f)}_d = \sum_{r=1} \v^{(f)}_r \lambda^{(f)}_r {\v^{(f)}_r}^T.
\end{equation}
For $\y^{(f)}(\x)$, let's assume a general decomposition as follows,
\begin{equation}
\label{eq:lmc2}
\y^{(f)}(\x) = \sum_{r=1}^\infty \b_r^{(f)} z_r^{(f)}\left(\x, \y_*^{(f-1)}(\x) \right),
\end{equation}
and place a GP prior for each $\z^{(f)}\left(\x, \y_*^{(f-1)}(\x) \right)$, \ie
\begin{equation}
z_r^{(f)}\left(\x, \y_*^{(f-1)}(\x) \right) \sim \mathcal{N}(0, k_{r}([\x, \y_*^{(f-1)}(\x) ], [\x', \y_*^{(f-1)}(\x') ])).
\end{equation}
The sum of GPs is still a GP. Likewise, a linear transformation of a GP is also a GP~\citep{rasmussen2003gaussian}.
From Eq.~\eqref{eq:lmc2}, we can derive 
\begin{equation}
	\y^{(f)}(\x) \sim \mathcal{N} \left(\0, \B^{(f)} \cov\left[\z(\x),\z(\x')\right] {\B^{(f)}}^T \right),
\end{equation}
\sloppy{where $\cov \left[\z(\x),\z(\x')\right]$ is the covariance between the multivariate GPs $\{z_r(\x,\y_*^{(f-1)}(\x))\}_{r=1}^\infty$.
We can further place a simplifying assumption,} 
\begin{equation}
\cov[\z(\x),\z(\x')] = \I \otimes  k\left( [\x, \y_*^{(f-1)}(\x) ], [\x', \y_*^{(f-1)}(\x') ] \right),
\end{equation}
where $\otimes$ is the Kronecker product. With this simplification, we can derive
\begin{equation}
\label{eq:sep2icm}
\y^{(f)}(\x) \sim \mathcal{N} \left(\0,  \sum_{r=1}^\infty \b_r^{(f)} {\b_r^{(f)}}^T k\left(([\x, \y_*^{(f-1)}(\x) ], [\x', \y_*^{(f-1)}(\x') ] \right) \right).
\end{equation}
If we let the bases in Eq.~\eqref{eq:sep2icm} be the product of the eigenvector and square root of eigenvalue in Eq.~\eqref{eq:eigen}, \ie $\b_r^{(f)} = \v^{(f)}_r \sqrt{\lambda^{(f)}_r}$,
we can clearly see that Eq.~\eqref{eq:sep2icm} has the exact kernel function of Eq.~\eqref{eq:sepInMatrix}. 
Note that Eq.~\eqref{eq:sep2icm} is achieved with a few simplifying assumptions. Thus, a covariance function of Eq.~\eqref{eq:deep gp kernel2} is implicitly a special case of the decomposition of Eq.~\eqref{eq:lmc2}. Consequently, we can say that Eq.~\eqref{eq:sep2icm} is equivalent to a GP with covariance function of the form of Eq.~\eqref{eq:deep gp kernel2}.

\section{Proof of Lemma~\ref{LEMMA2} } 
\label{ap:proof l2}
For a general kernel of 
$k_y^{(f)}(\b^{(f-1)} z_*^{(f-1)}(\x), \b^{(f-1)} z_*^{(f-1)}(\x'))$, 
it is the valid stationary kernel iff
\begin{equation}
\begin{aligned}
 k_y^{(f)} & (\b^{(f-1)} z_*^{(f-1)}(\x), \b^{(f-1)} z_*^{(f-1)}(\x'))\\
& = 	\int_{\mathbb{R}^d} \cos\left(\pmb\omega^T \left(\b^{(f-1)} z_*^{(f-1)}(\x) - \b^{(f-1)} z_*^{(f-1)}(\x') \right) \right) F(d \pmb\omega ), 
\end{aligned}
\end{equation}
where $F$ is a positive finite measure~\citep{genton2001classes}. Let $\pmb\omega^T \b^{(f-1)} = \pmb\phi^T$, we have
\begin{equation}
\begin{aligned}
& k_y^{(f)}(\b^{(f-1)} z_*^{(f-1)}(\x), \b^{(f-1)} z_*^{(f-1)}(\x'))\\
& = 	\int_{\mathbb{R}^d} \cos\left(\pmb\phi^T \left( z_*^{(f-1)}(\x) -  z_*^{(f-1)}(\x') \right) \right) F( \b^{(f)} d \pmb\phi)\\
& =	\int_{\mathbb{R}^d} \cos\left(\pmb\phi^T \left( z_*^{(f-1)}(\x) -  z_*^{(f-1)}(\x') \right) \right) \hat{F}( d \pmb\phi)\\
& = k_z^{(f)}(z_*^{(f-1)}(\x), z_*^{(f-1)}(\x')).
\end{aligned}
\end{equation}
$\hat{F}(d \pmb\phi)$ must exist because $ \b^{(f)} d \pmb\phi$ represents a subset of $d \pmb\phi$ and $\hat{F}$ is an barbarity positive measure. 
%$d \pmb\phi$ is a low-dimensional projection of $d \pmb\omega$, an alternative positive measure $\hat{F}(d \pmb\phi)$ must exist for the subsets of $d \pmb\omega$ recovered by $d \pmb\phi$.
Thus, $k_z^{(f)}(z_*^{(f-1)}(\x), z_*^{(f-1)}(\x'))$ exist and it is also stationary.
%\begin{equation}
%\begin{aligned}
%& 	\int_{\mathbb{R}^d} \cos\left(\pmb\phi^T \left( z_*^{(f-1)}(\x) -  z_*^{(f-1)}(\x') \right) \right) \hat{F}( d \pmb\phi)\\
%& = k_z^{(f)}(z_*^{(f-1)}(\x), z_*^{(f-1)}(\x')),
%\end{aligned}
%\end{equation}
%which is certainly stationary.

\cmt{
\section{Proof of Lemma~\ref{LEMMA1} } 
%\label{ap:proof l2}
We provide a proof of Lemma~\ref{LEMMA1} here.
For celerity, let's omit the multi-fidelity data and consider a simple case,
\begin{equation}
\cov[\y^{(f)}(\x), \y^{(f)}(\x')] = k_d(i,j) k_x(\x,\x')
\end{equation}
where $k_d$ is the function 

First assume that $\y^{(f)}(\x)$ can be decomposed as follows,
\begin{equation}
\y^{(f)}(\x) = \sum_i \b_i^{(f)} z_i^{(f)}\left(\x, \y_*^{(f-1)}(\x) \right)
\end{equation}
Assume that each $\z^{(f)}\left(\x, \y_*^{(f-1)}(\x) \right)$ is a GP, \ie
\begin{equation}
\z_r^{(f)}\left(\x, \y_*^{(f-1)}(\x) \right) \sim \mathcal{N}(\0, k_{zr}([\x, \y_*^{(f-1)}(\x) ], [\x', \y_*^{(f-1)}(\x') ]))
\end{equation}
The sum of GPs is still a GP. Likewise, a linear transformation of a GP is also a GP~\citep{rasmussen2003gaussian}. Thus, $\y^{(f)}(\x)$ is a GP as
\begin{equation}
\y^{(f)}(\x) \sim \mathcal{N} \left(\0, \B^{(f)} \cov[\z(\x),\z(\x')] {\B^{(f)}}^T \right),
\end{equation}
where $\cov[\z(\x),\z(\x')]$ is the covariance the multivariate GP $\z(\x)$.
Let $\cov[\z(\x),\z(\x')] = \I \otimes  k_{z}([\x, \y_*^{(f-1)}(\x) ], [\x', \y_*^{(f-1)}(\x') ])$.
With this simplification, 
\begin{equation}
\label{eq:sep2icm}
\y^{(f)}(\x) \sim \mathcal{N} \left(\0,  \sum_r \b_r^{(f)} {\b_r^{(f)}}^T k_{z}([\x, \y_*^{(f-1)}(\x) ], [\x', \y_*^{(f-1)}(\x') ]) \right),
\end{equation}
Recognize that this equation is equivalent to 

For a kernel function having the Eq.\eqref{eq:deep gp kernel2}, we can directly write the covariance of the whole vector $\y^{(f)}(\x)$ as 
\begin{equation}
\label{eq:sepInMatrix}
\cov[\y^{(f)}(\x),\y^{(f)}(\x')] = \K_d \cdot k_{z}([\x, \y_*^{(f-1)}(\x) ], [\x', \y_*^{(f-1)}(\x') ])
\end{equation}
where $[\K^{(f)}_d]_{ij}=k^({f})_d(i,j)$ is the covariance matrix of outputs. Since $\K^{(f)}_d$ is guaranteed to be p.s.d., we have the eigendecomposition, 
$\K^{(f)}_d = \sum_r \v^{(f)}_r \lambda^{(f)}_r {\v^{(f)}_r}^T$.
Now, let the bases in Eq.~\eqref{eq:sep2icm} be $\b_r^{(f)} = \v^{(f)}_r \sqrt{\lambda^{(f)}_r}$, we can clearly see that Eq.~\eqref{eq:sep2icm} has the exact kernel function as Eq.~\eqref{eq:sepInMatrix}.
}
	
\section{Proof of Theorem \ref{THEOREM2}}
\label{ap:proof t2}
%We want to prove that $\y^{(f)}(\x)=\B^{(f)} \hat{\g}^{(f)}\left(\x,\z_*^{(f-1)}(\x)\right)$,
%where 
%
%\begin{equation}
%\begin{aligned}
%\B^{(f)} \z^{(f)}(\x) & = \g^{(f)}\left(\x, \B^{(f-1)} \z_*^{(f-1)}(\x)\right)\\
%\z^{(f)}(\x) & = {\B^{(f)}}^T \g^{(f)}\left(\x, \B^{(f-1)} \z_*^{(f-1)}(\x)\right)\\
%\z^{(f)}(\x) & = \hat{\g}^{(f)}\left(\x,\z_*^{(f-1)}(\x)\right),\\
%\end{aligned}
%\label{eq:deep lmc1}
%\end{equation}
By the LMC formulation of Eq.~\eqref{eq:lmc multi}, we know that $\y^{(f)}(\x)=\g^{(f)}\left(\x, \B^{(f-1)} \z_*^{(f-1)}(\x)\right)$ is a multivariate GP by its definition (a linear transformation of a GP is still a GP). 
%Similarly, $\g^{(f)}\left(\x, \B^{(f-1)} \z_*^{(f-1)}(\x)\right)$ is also a GP as a result of linear transformation.
Let's denote the unknown kernel function of 
$\g^{(f)}\left(\x, \B^{(f-1)} \z_*^{(f-1)}(\x)\right)$ via a general kernel function
\[
\cov \left[y_i^{(f)}(\x),y_i^{(f)}(\x) \right] = \textit{k} \left([i, \x,\B^{(f-1)} \z_*^{(f-1)}(\x)], [j, \x',\B^{(f-1)} \z_*^{(f-1)}(\x')] \right),
\]
which can be further expanded as
\begin{equation}
\begin{aligned}
\label{eq:compact kernel}
& k\left(\left[i, \x,\B^{(f-1)} \z_*^{(f-1)}(\x)\right], \left[j, \x',\B^{(f-1)} \z_*^{(f-1)}(\x')\right] \right)\\
%&= \left\langle \varphi([\x,\y_*^{(f-1)}(\x)]), \varphi([\x',\y_*^{(f-1)}(\x')])  \right\rangle_{\mathcal{V}}\\
&= \left\langle \varphi(\left[i, \x,\B^{(f-1)} \z_*^{(f-1)}(\x) \right]), \varphi(\left[j, \x',\B^{(f-1)} \z_*^{(f-1)}(\x) \right]) \right\rangle_{\mathcal{V}}\\
&= \left\langle \hat{\varphi}(\left[i, \x, \z_*^{(f-1)}(\x)\right]), \hat{\varphi}(\left[j, \x', \z_*^{(f-1)}(\x)\right]) \right\rangle_{\mathcal{V}}\\
&= \hat{k}\left( \left[ i, \x, \z_*^{(f-1)}(\x) \right], \left[,\x', \z_*^{(f-1)}(\x') \right] \right),
\end{aligned}
\end{equation}
where $\varphi$ is an implicit feature mapping, $ \left\langle \cdot, \cdot  \right\rangle_{\mathcal{V}}$ is a proper inner product in the inner product space $\mathcal{V}$, $\hat{\varphi}$ is the composite function of $\varphi$ absorbing $\B^{(f-1)}$ and $\hat{k}$ is the composite kernel function. 
$\hat{\varphi}$ always exist as the input space ($[i, \x, \z_*^{(f-1)}(\x)]$) is a subspace of $[i, \x, \y_*^{(f-1)}(\x)]$.
Similarly, as $k$ satisfies Mercer's condition, $\hat{k}$ also satisfies Mercer's condition and thus $\hat{k}$ must exist.
% and $\hat{k}$ always exist due to the inner product and $k$ satisfies Mercer's condition.
Thus $\g^{(f)}\left(\x, \B^{(f-1)} \z_*^{(f-1)}(\x)\right)$ have a compact representation $\tilde{g}^{(f)}\left(\x, \z_*^{(f-1)}(\x)\right)$. 
For the independence,
\begin{equation}
\begin{aligned}
\cov & \left[ \hat{g}_i( \x, \z_*^{(f-1)}(\x) ) , \hat{g}_j( \x, \z_*^{(f-1)}(\x) )  \right]\\
& = {\b_i^{(f)}}^T \cov\left[ \tilde{g}_i( \x, \z_*^{(f-1)}(\x) ) , \tilde{g}_j( \x, \z_*^{(f-1)}(\x) )  \right] \b_j^{(f)}
&=0,
\end{aligned}
\end{equation} 
because $\b_i^{(f)}$ and $\b_j^{(f)}$ are orthogonal and thus $\hat{g}_i( \x, \z_*^{(f-1)}(\x) )$ can be treated as independent univariate GP, which match the independent assumption of $\z^{(f)}(\x)$.

\cmt{
\section{Proof of Theorem \ref{THEOREM1}}
\label{ap:proof t1}
Assuming that $\g^{(f)}$ is a multivariate GP which admit a LMC presentation, we have
% it has a separable structure, we have,
%\begin{equation}
%\y^{(f)}(\x)=\g^{(f)}(\x,\y_*(\x)) = \mathcal{GP} \left(\m(\x), k_s(i,j) \cdot k(\x, \x', \y_*^{(f-1)}(\x),\y_*^{(f-1)}(\x') )\right)
%\end{equation}
%where $i,j$ indicate the particular dimensional indexes for the output, $\m(\x)$ is the mean function and $k_s$ is kernel function for the between-output correlations. $\m(\x)$ is normally assumed zero function after normalizing the data. 
%Due to the separable structure, we can write the between-output correlation in a matrix form as,
\begin{equation}
\label{eq:cov right}
%\cov[\y^{(f)}(\x),\y^{(f)}(\x')] = \K_s \cdot k(\x, \x', \y_*^{(f-1)}(\x),\y_*^{(f-1)}(\x'))
\cov[\g^{(f)}(\x,\y_*^{(f-1)}(\x)), \g^{(f)}(\x',\y_*^{(f-1)}(\x'))] = \sum_r \K_{sr} \cdot k_r(\x, \x', \y_*^{(f-1)}(\x),\y_*^{(f-1)}(\x'))
\end{equation}
where $\K_{sr}$ is the r-th between-output correlation matrix. 
Based on the LMC formulation of Eq.\eqref{eq:lmc}, the covariance structure for $\y^{(f)}(\x)$ must have the following form:
%Using the LMC formulation of Eq.\eqref{eq:lmc} and , for $\y^{(f)}(\x)$, we have,
\begin{equation}
\label{eq:cov left}
\begin{aligned}
\cov[\y^{(f)}(\x),\y^{(f)}(\x')] &= \EE[\y^{(f)}(\x) {\y^{(f)}}^T(\x')] - \EE[\y^{(f)}(\x)] \EE[\y^{(f)}(\x')] \\
&=\EE[ \B^{(f)} \z^{(f)}(\x) {\z^{(f)}}^T(\x') {\B^{(f)}}^T]\\
&= \B^{(f)} \cov[ \z^{(f)}(\x),\z^{(f)}(\x')] {\B^{(f)}}^T.
\end{aligned}
\end{equation}
For LMC, $\K_{sr}$ is the covariance matrix and can be decomposed as $\K_{sr} = \v_{sr} \lambda_{sr} \v_{sr}^T$ via eigendecomposition. 
%Here $\lambda_s$ is diagonal and $\V_s$ is orthonormal, \ie $\V_{sr} \V_{sr}^T =\I $.
Let $B^{(f)} = [\v_{s1},\cdots,\v_{sr}] = \V_s$ and substitute Eq.\eqref{eq:cov left} into Eq.\eqref{eq:cov right}, we have
\begin{equation}
\begin{aligned}
\label{eq:cov 2}
\V_s \cov[ \z^{(f)}(\x),\z^{(f)}(\x')] \V_s^T &= \sum_r \K_{sr} \cdot k_r(\x, \x', \y_*^{(f-1)}(\x),\y_*^{(f-1)}(\x'))\\
 \cov[ \z^{(f)}(\x),\z^{(f)}(\x')] &= \sum_r \V_s^T \K_{sr} \V_s \cdot k_r(\x, \x', \y_*^{(f-1)}(\x),\y_*^{(f-1)}(\x'))\\
\cov[ \z^{(f)}(\x),\z^{(f)}(\x')] &= \sum_r \Lambda_{sr} \cdot k_r(\x, \x', \y_*^{(f-1)}(\x),\y_*^{(f-1)}(\x')).\\
\end{aligned}
\end{equation}
This equation shows that $\z^{(f)}(\x)$ can be decomposed into independent univariate GP since $k_r$ are assumed independent by the LMC.
%Since $\Lambda_s$ is diagonal, $\cov[ \z^{(f)}(\x),\z^{(f)}(\x')]$ is also a diagonal matrix, indicating that it is sufficient to say that $\z^{(f)}(\x)$ can be decomposed into independent univariate GP.
Note that the kernel function is still based on the high-dimensional $\y_*^{(f-1)}(\x)$. Due to the LMC assumption, we have $\y_*^{(f-1)}(\x) = \B^{(f-1)} \z_*^{(f-1)}(\x) $. The kernel function can now be updated as
\begin{equation}
\begin{aligned}
\label{eq:compact kernel}
 & k_r\left(\x, \x', \y_*^{(f-1)}(\x),\y_*^{(f-1)}(\x')\right)\\
 &= \left\langle \varphi([\x,\y_*^{(f-1)}(\x)]), \varphi([\x',\y_*^{(f-1)}(\x')])  \right\rangle_{\mathcal{V}}\\
 &= \left\langle \varphi([\x,\B^{(f-1)} \z_*^{(f-1)}(\x)]), \varphi([\x',\B^{(f-1)} \z_*^{(f-1)}(\x)]) \right\rangle_{\mathcal{V}}\\
 &= \left\langle \hat{\varphi}([\x, \z_*^{(f-1)}(\x)]), \hat{\varphi}([\x', \z_*^{(f-1)}(\x)]) \right\rangle_{\mathcal{V}}\\
 &= \hat{k}_r\left(\x, \x', \z_*^{(f-1)}(\x),\z_*^{(f-1)}(\x')\right),\\
\end{aligned}
\end{equation}
where $\varphi$ is an implicit feature mapping, $ \left\langle \cdot, \cdot  \right\rangle_{\mathcal{V}}$ is a proper inner product in the inner product space $\mathcal{V}$, $\hat{\varphi}$ is the composite function of $\varphi$ absorbing $\B^{(f-1)}$ and $\hat{k}$ is the composite kernel function. $\hat{\varphi}$, and $\hat{k}$ always exist due to the inner product and $k$ satisfies Mercer's condition. Substituting Eq.\eqref{eq:compact kernel} into Eq.\eqref{eq:cov 2}, we have
\begin{equation}
\cov[ \z^{(f)}(\x),\z^{(f)}(\x')] = \sum_r \Lambda_{sr} \cdot  \hat{k}_r\left(\x, \x', \z_*^{(f-1)}(\x),\z_*^{(f-1)}(\x')\right),
\end{equation}
which is theorem \ref{THEOREM1}: $\y^{(f)}(\x)$ can be decomposed into several independent univariate GP given the LMC assumptions.

%	\section{Proof of lemma \ref{LEMMA1}}
%	Given a trained deep coregionalization, the posterior is a sum over many linear transformations of GPs.
%	Let $\{\z^{(f)}_*\}_{f=1}^F$ denote the posterior given a new input $\x_*$, posterior of the highest fidelity is 
%	\begin{equation}
%		\y^{(F)}(\x_*) &= \sum_{f=1}^F \B^{(f)} \z^{(f)}(\x_*).
%	\end{equation}
%	The expectation is 
%	\begin{equation}
%	\EE[\y^{(F)}(\x)] &= \sum_{f=1}^F \B^{(f)}\EE[\z^{(f)}(\x)].
%	\end{equation}
%	The variance is 
%	\begin{equation}
%	\EE[\y^{(F)}(\x) - ] &= \sum_{f=1}^F \B^{(f)}\EE[\z^{(f)}(\x)].
%	\end{equation}
}
\section{Actual Field Predictions for Two-fidelity Experiments}
\label{app:actual predictions lv2}
Six randomly selected actual predictive fields for Poisson's equation, the heat equation and Burger's equation for all competing methods using 256 fidelity-1 samples, 64 fidelity-2 samples, and $R=8$ are shown in Figs.~\ref{ap:lv2_1}, \ref{ap:lv2_2}, and \ref{ap:lv2_3}.
\begin{figure}[h]
	\centering
	\includegraphics[width=0.6\textwidth]{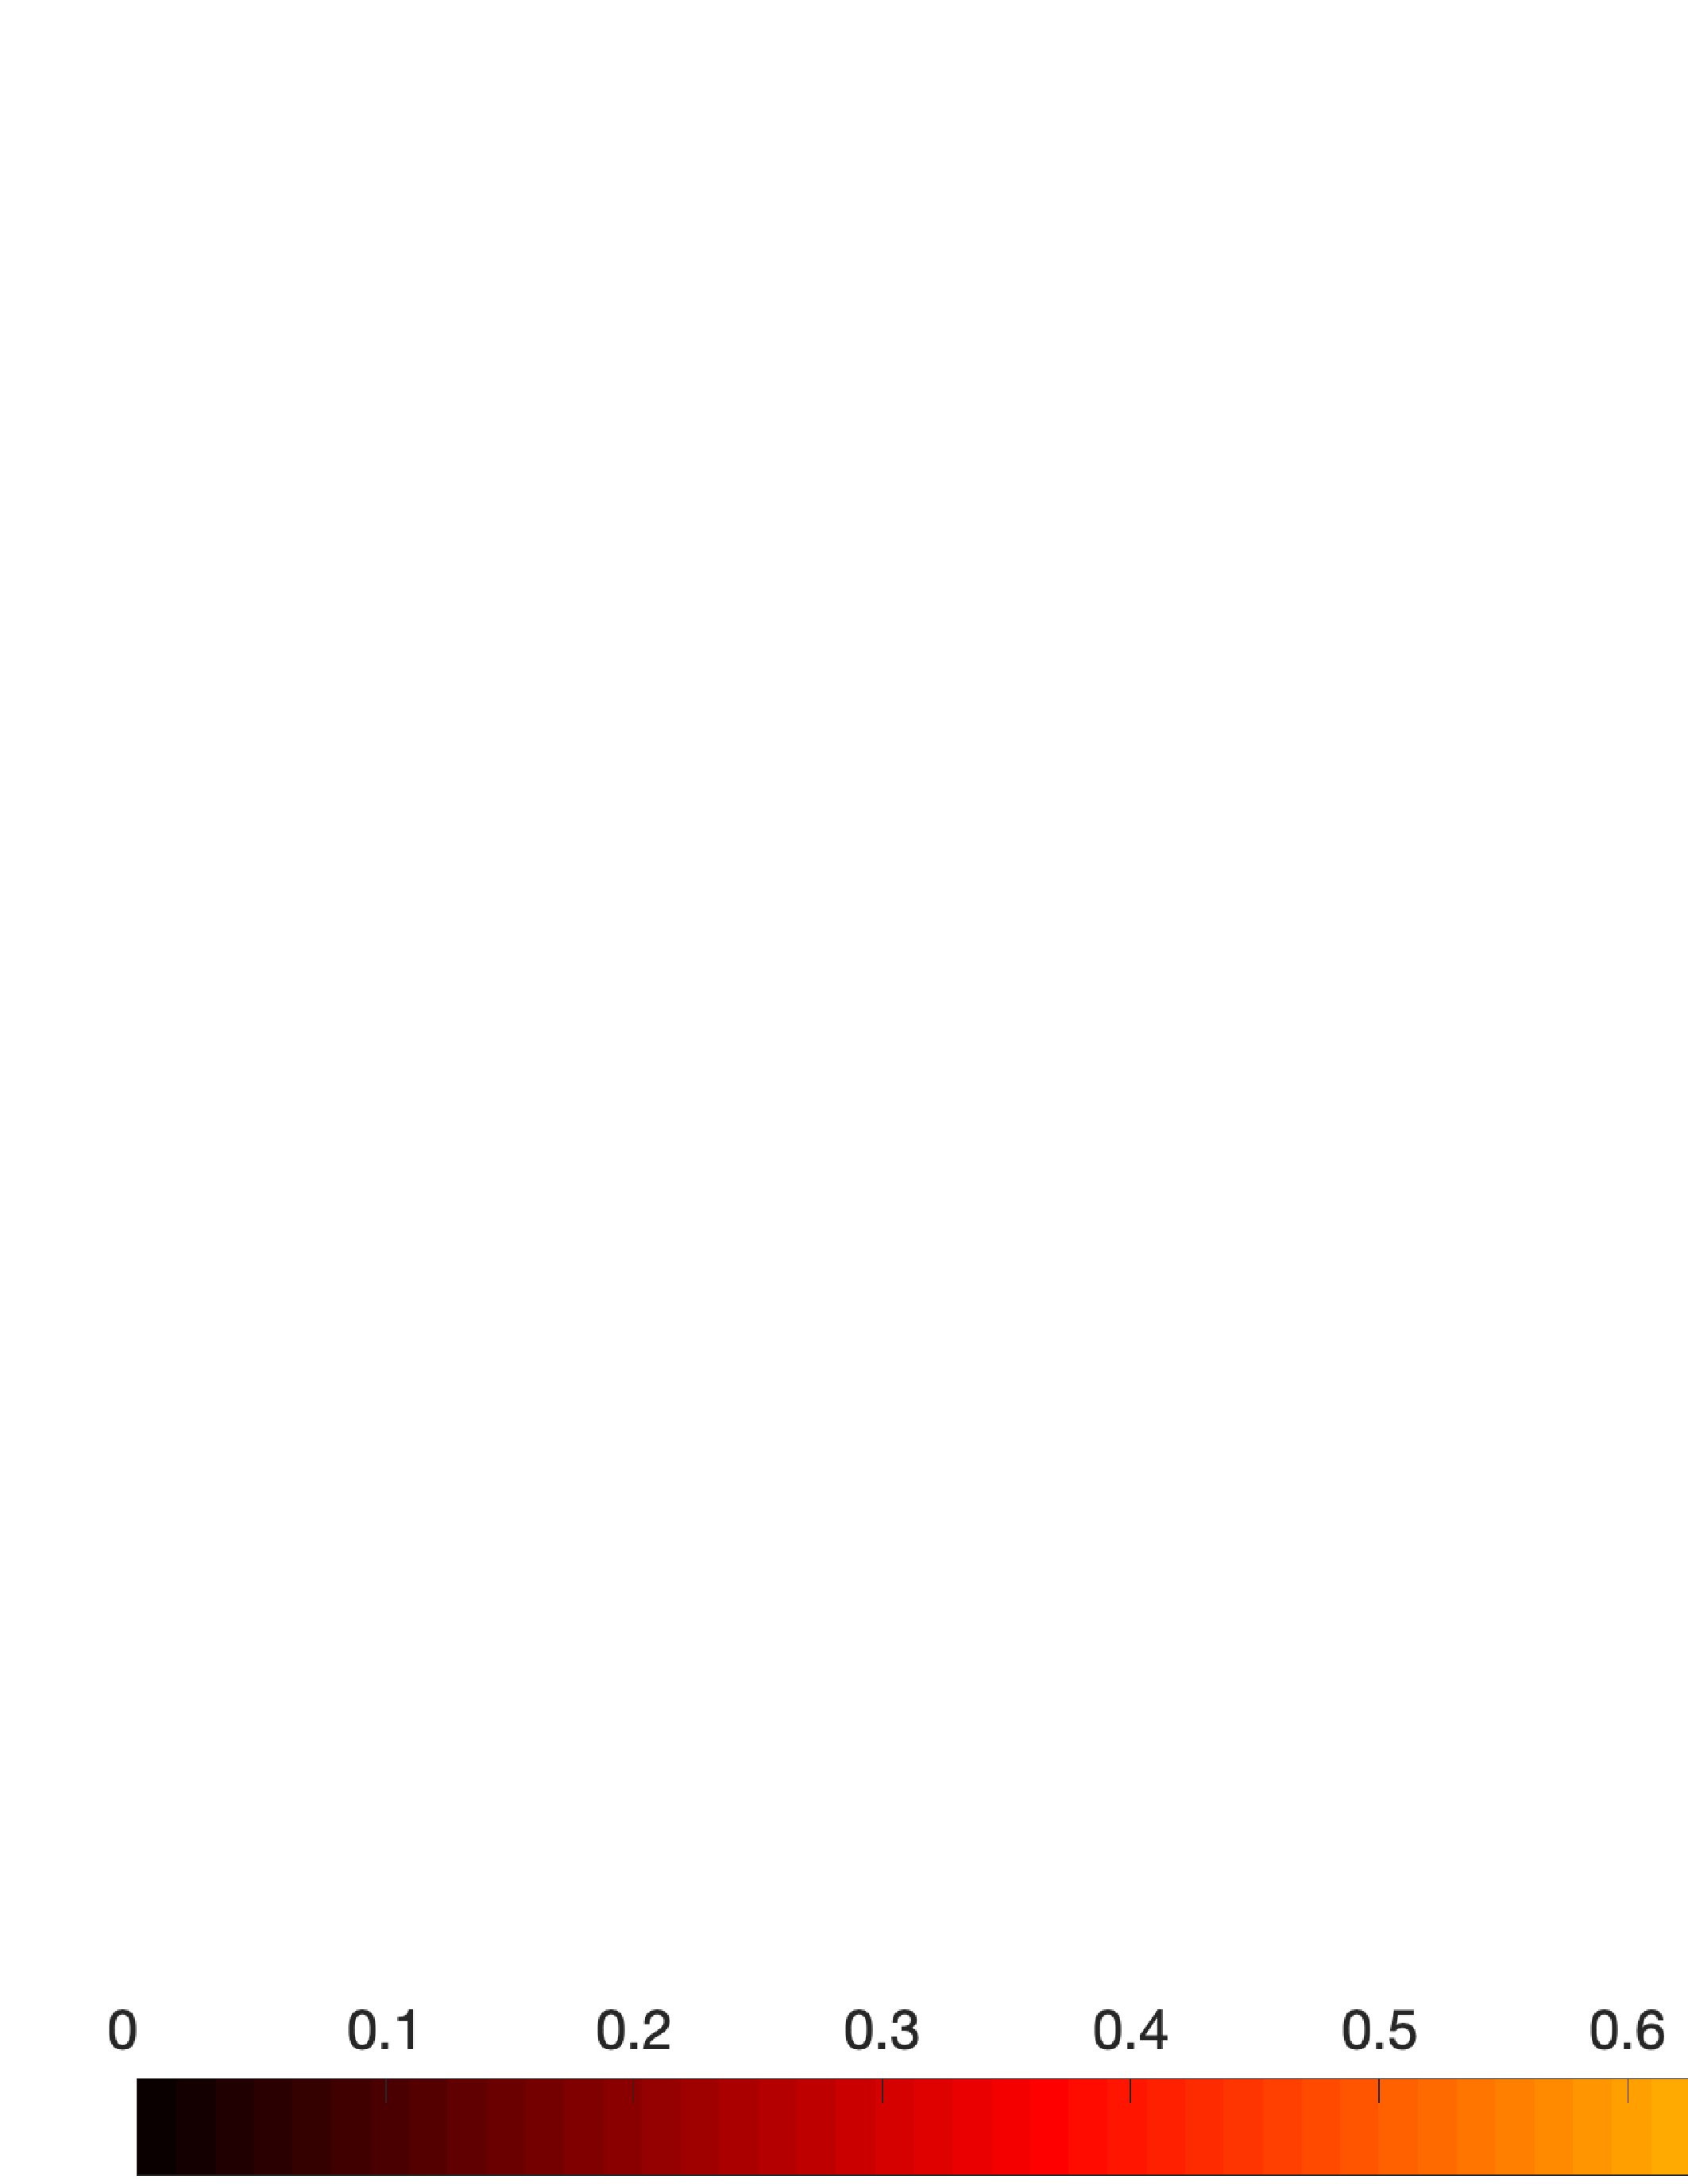}
	\includegraphics[width=\textwidth]{./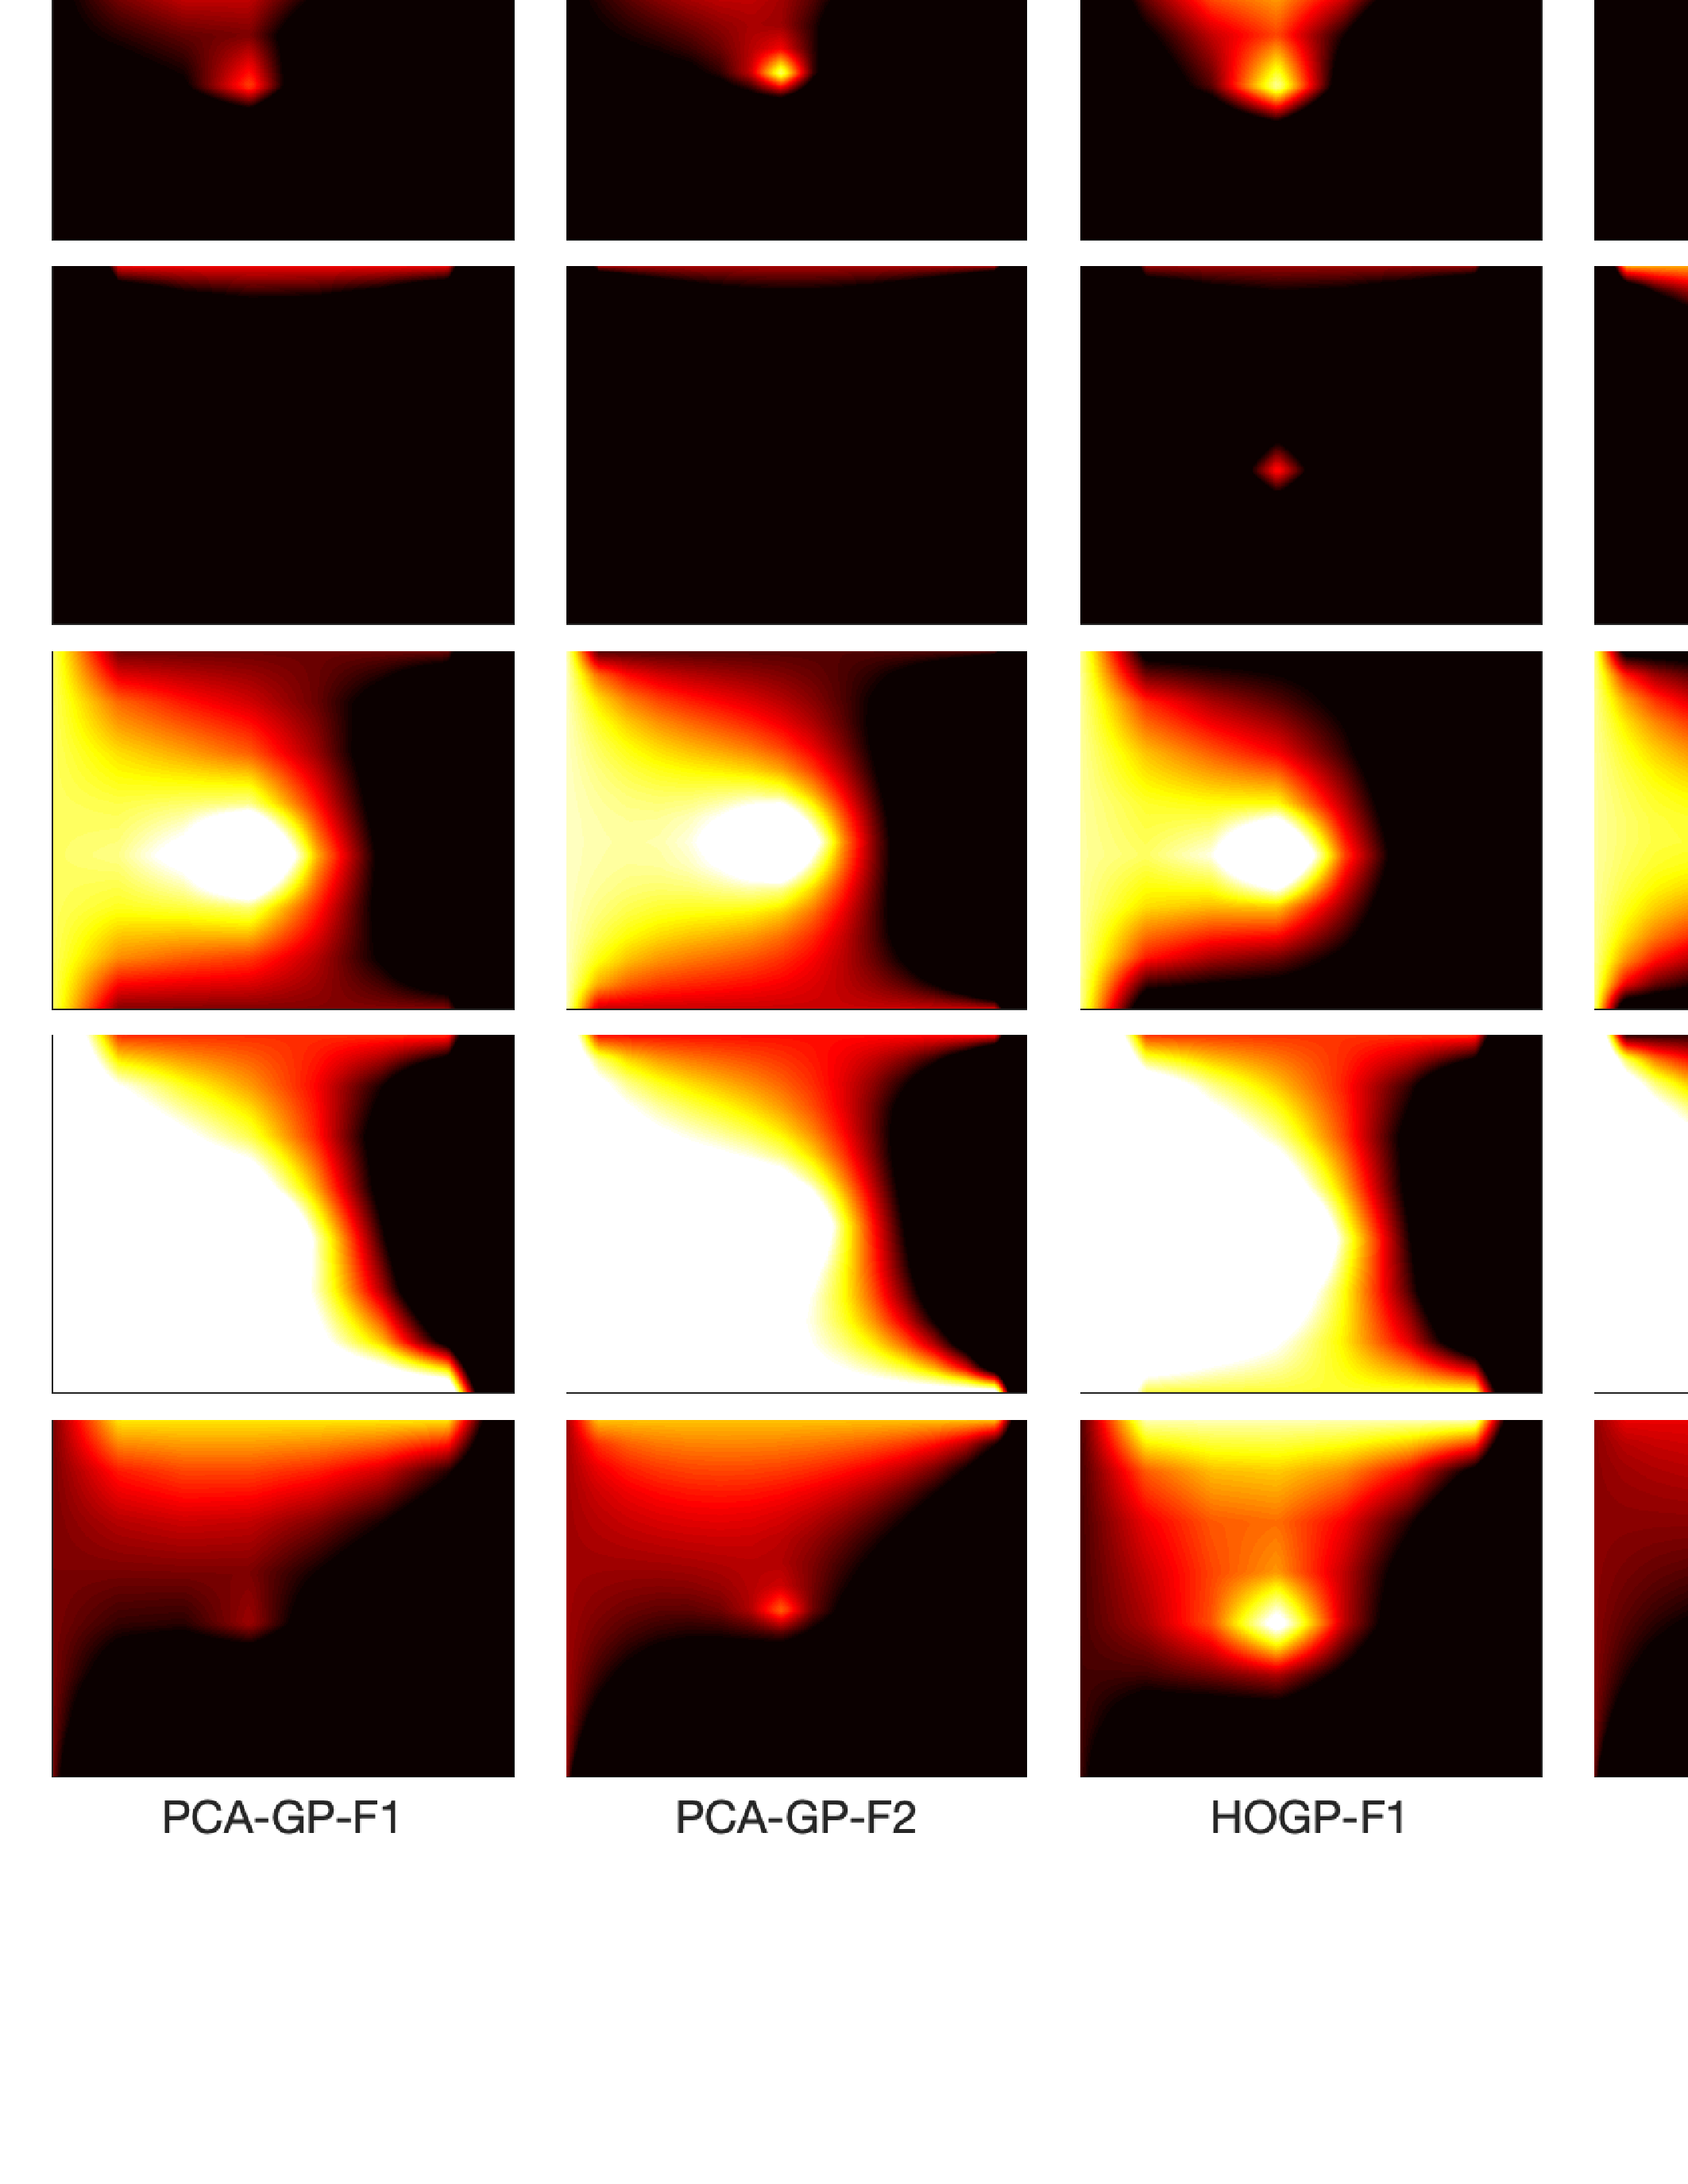}
	\caption{Actual predictive mean fields for Poisson's equation using 256 fidelity-1 samples, 64 fidelity-2 samples, and $R=8$.}
	\label{ap:lv2_1}
\end{figure}

\begin{figure}[h]
	\centering
	\includegraphics[width=0.6\textwidth]{./fig_v2/instHeatMapBar.eps}
	\includegraphics[width=\textwidth]{./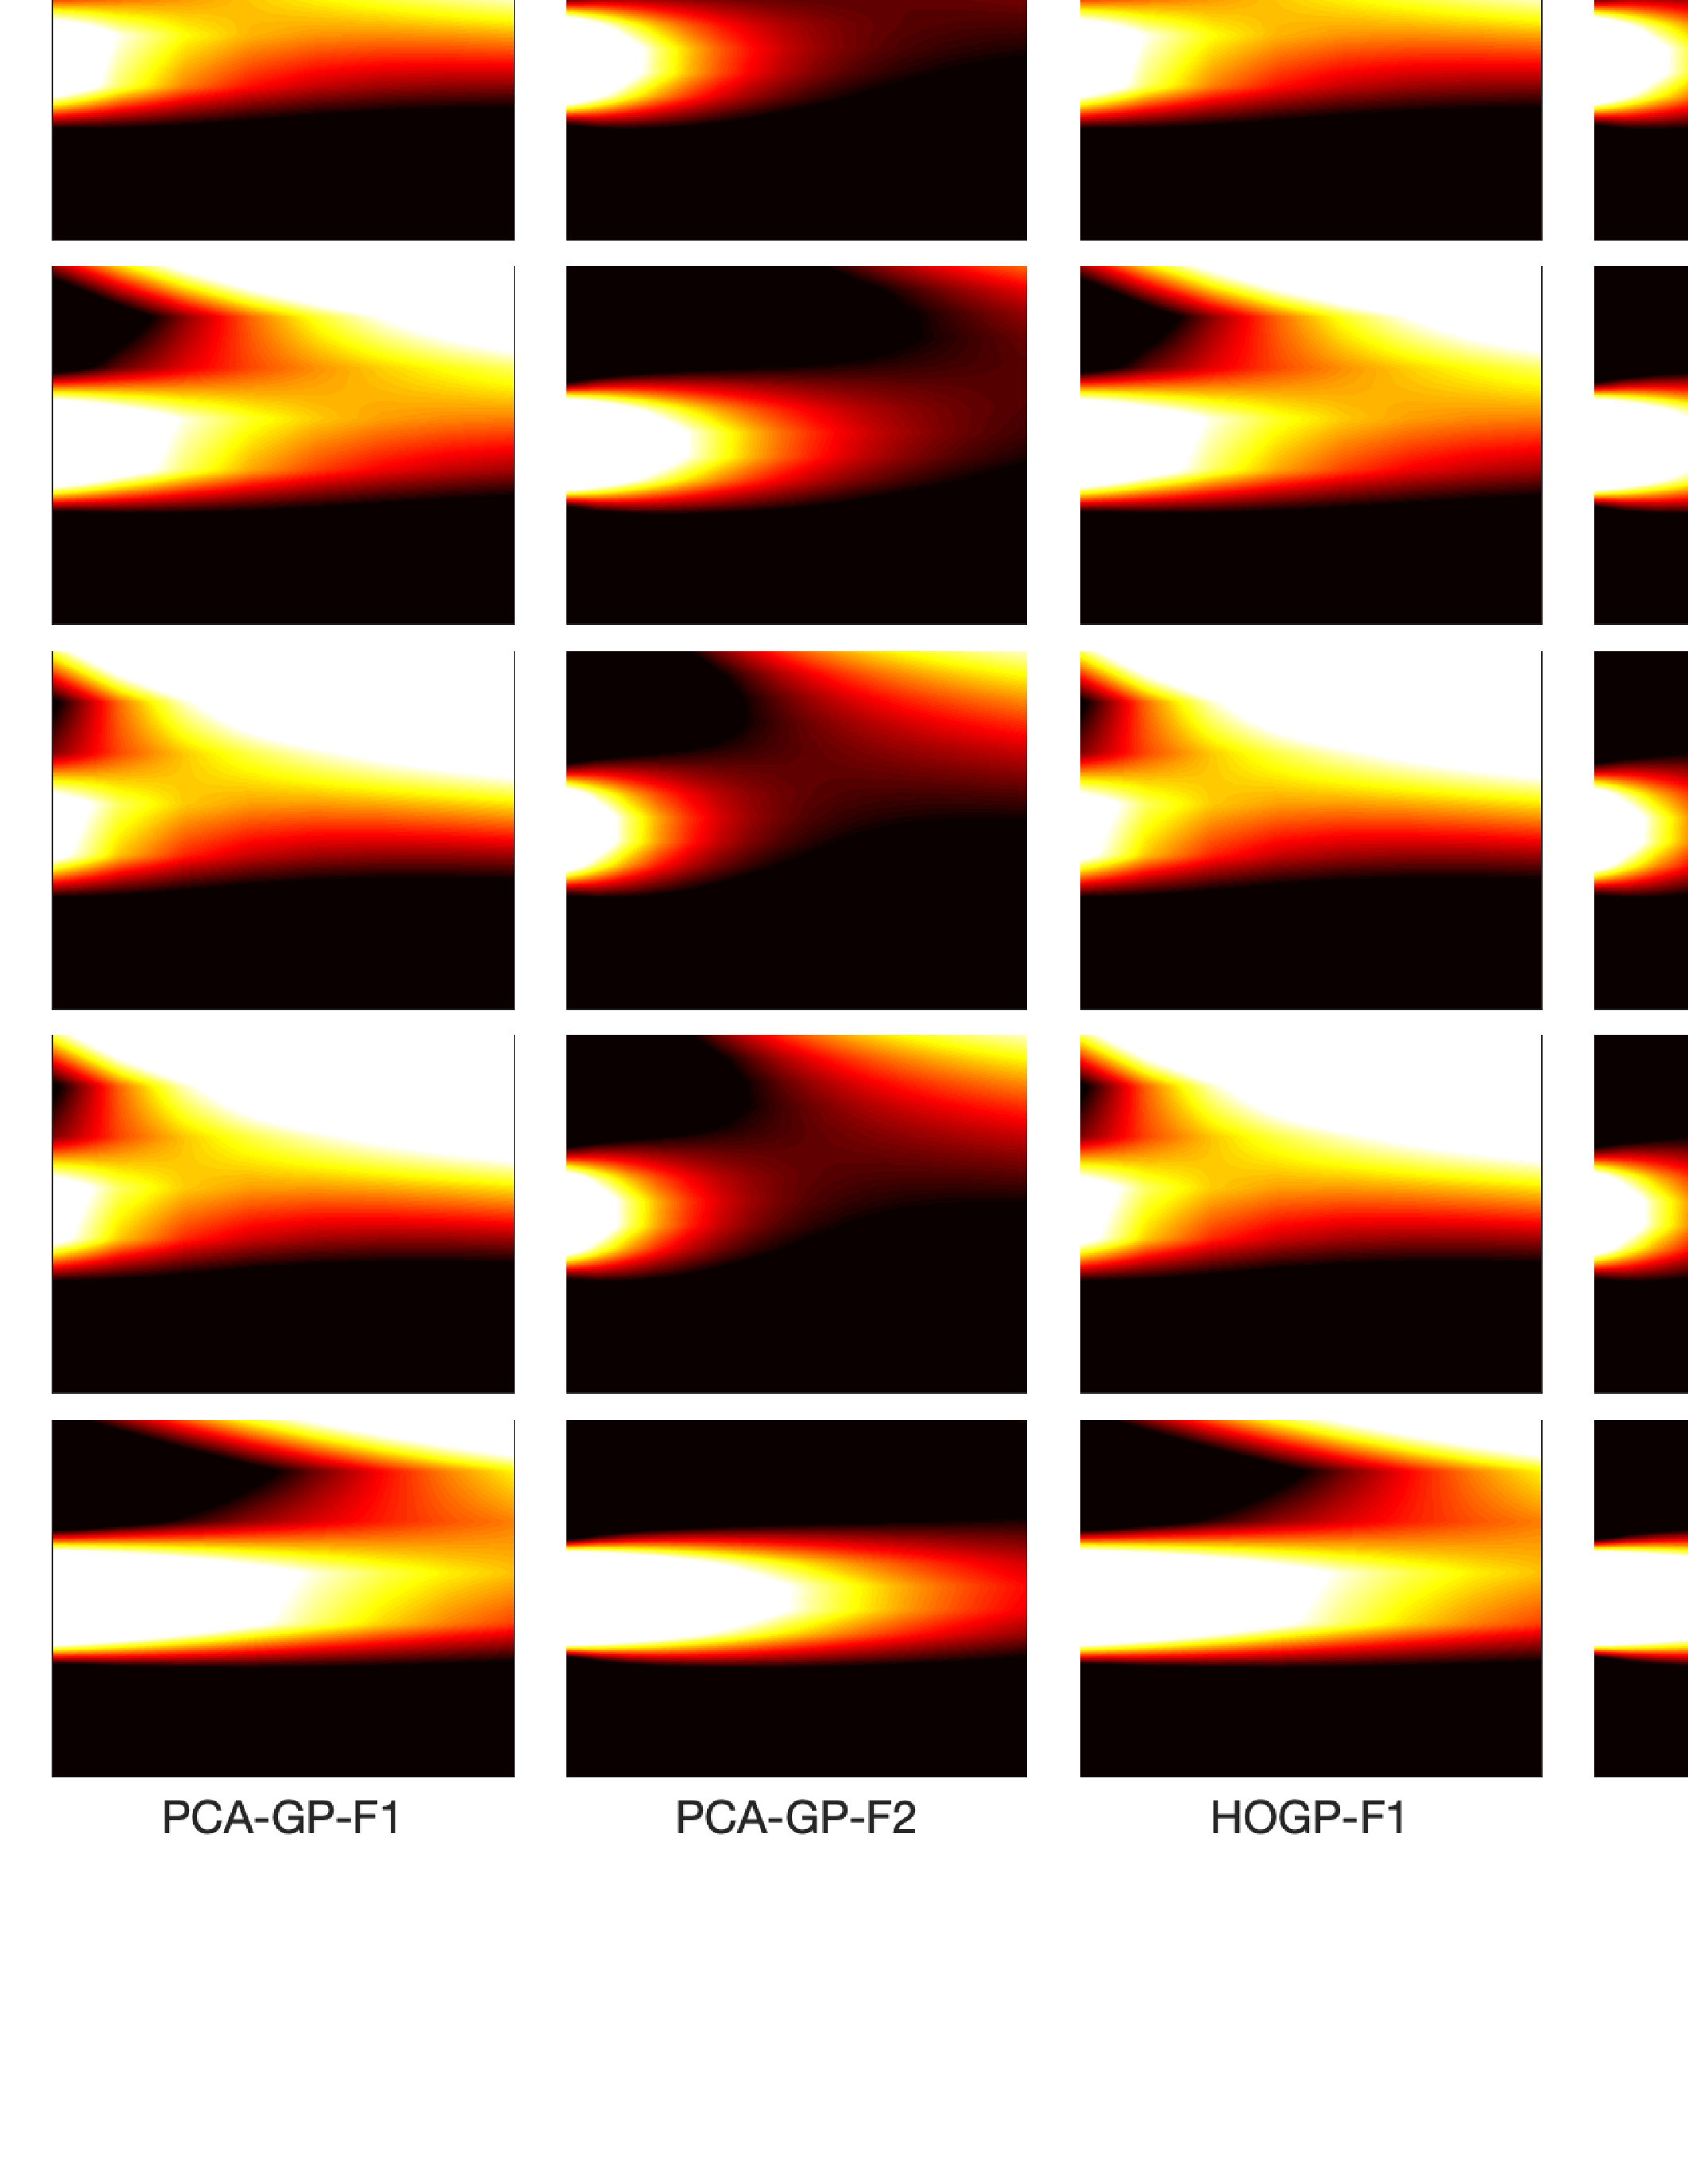}
	\caption{Actual predictive mean fields for heat equation using 256 fidelity-1 samples, 64 fidelity-2 samples, and $R=8$.}
	\label{ap:lv2_2}
\end{figure}

\begin{figure}[h]
	\centering
	\includegraphics[width=0.6\textwidth]{./fig_v2/instHeatMapBar.eps}
	\includegraphics[width=\textwidth]{./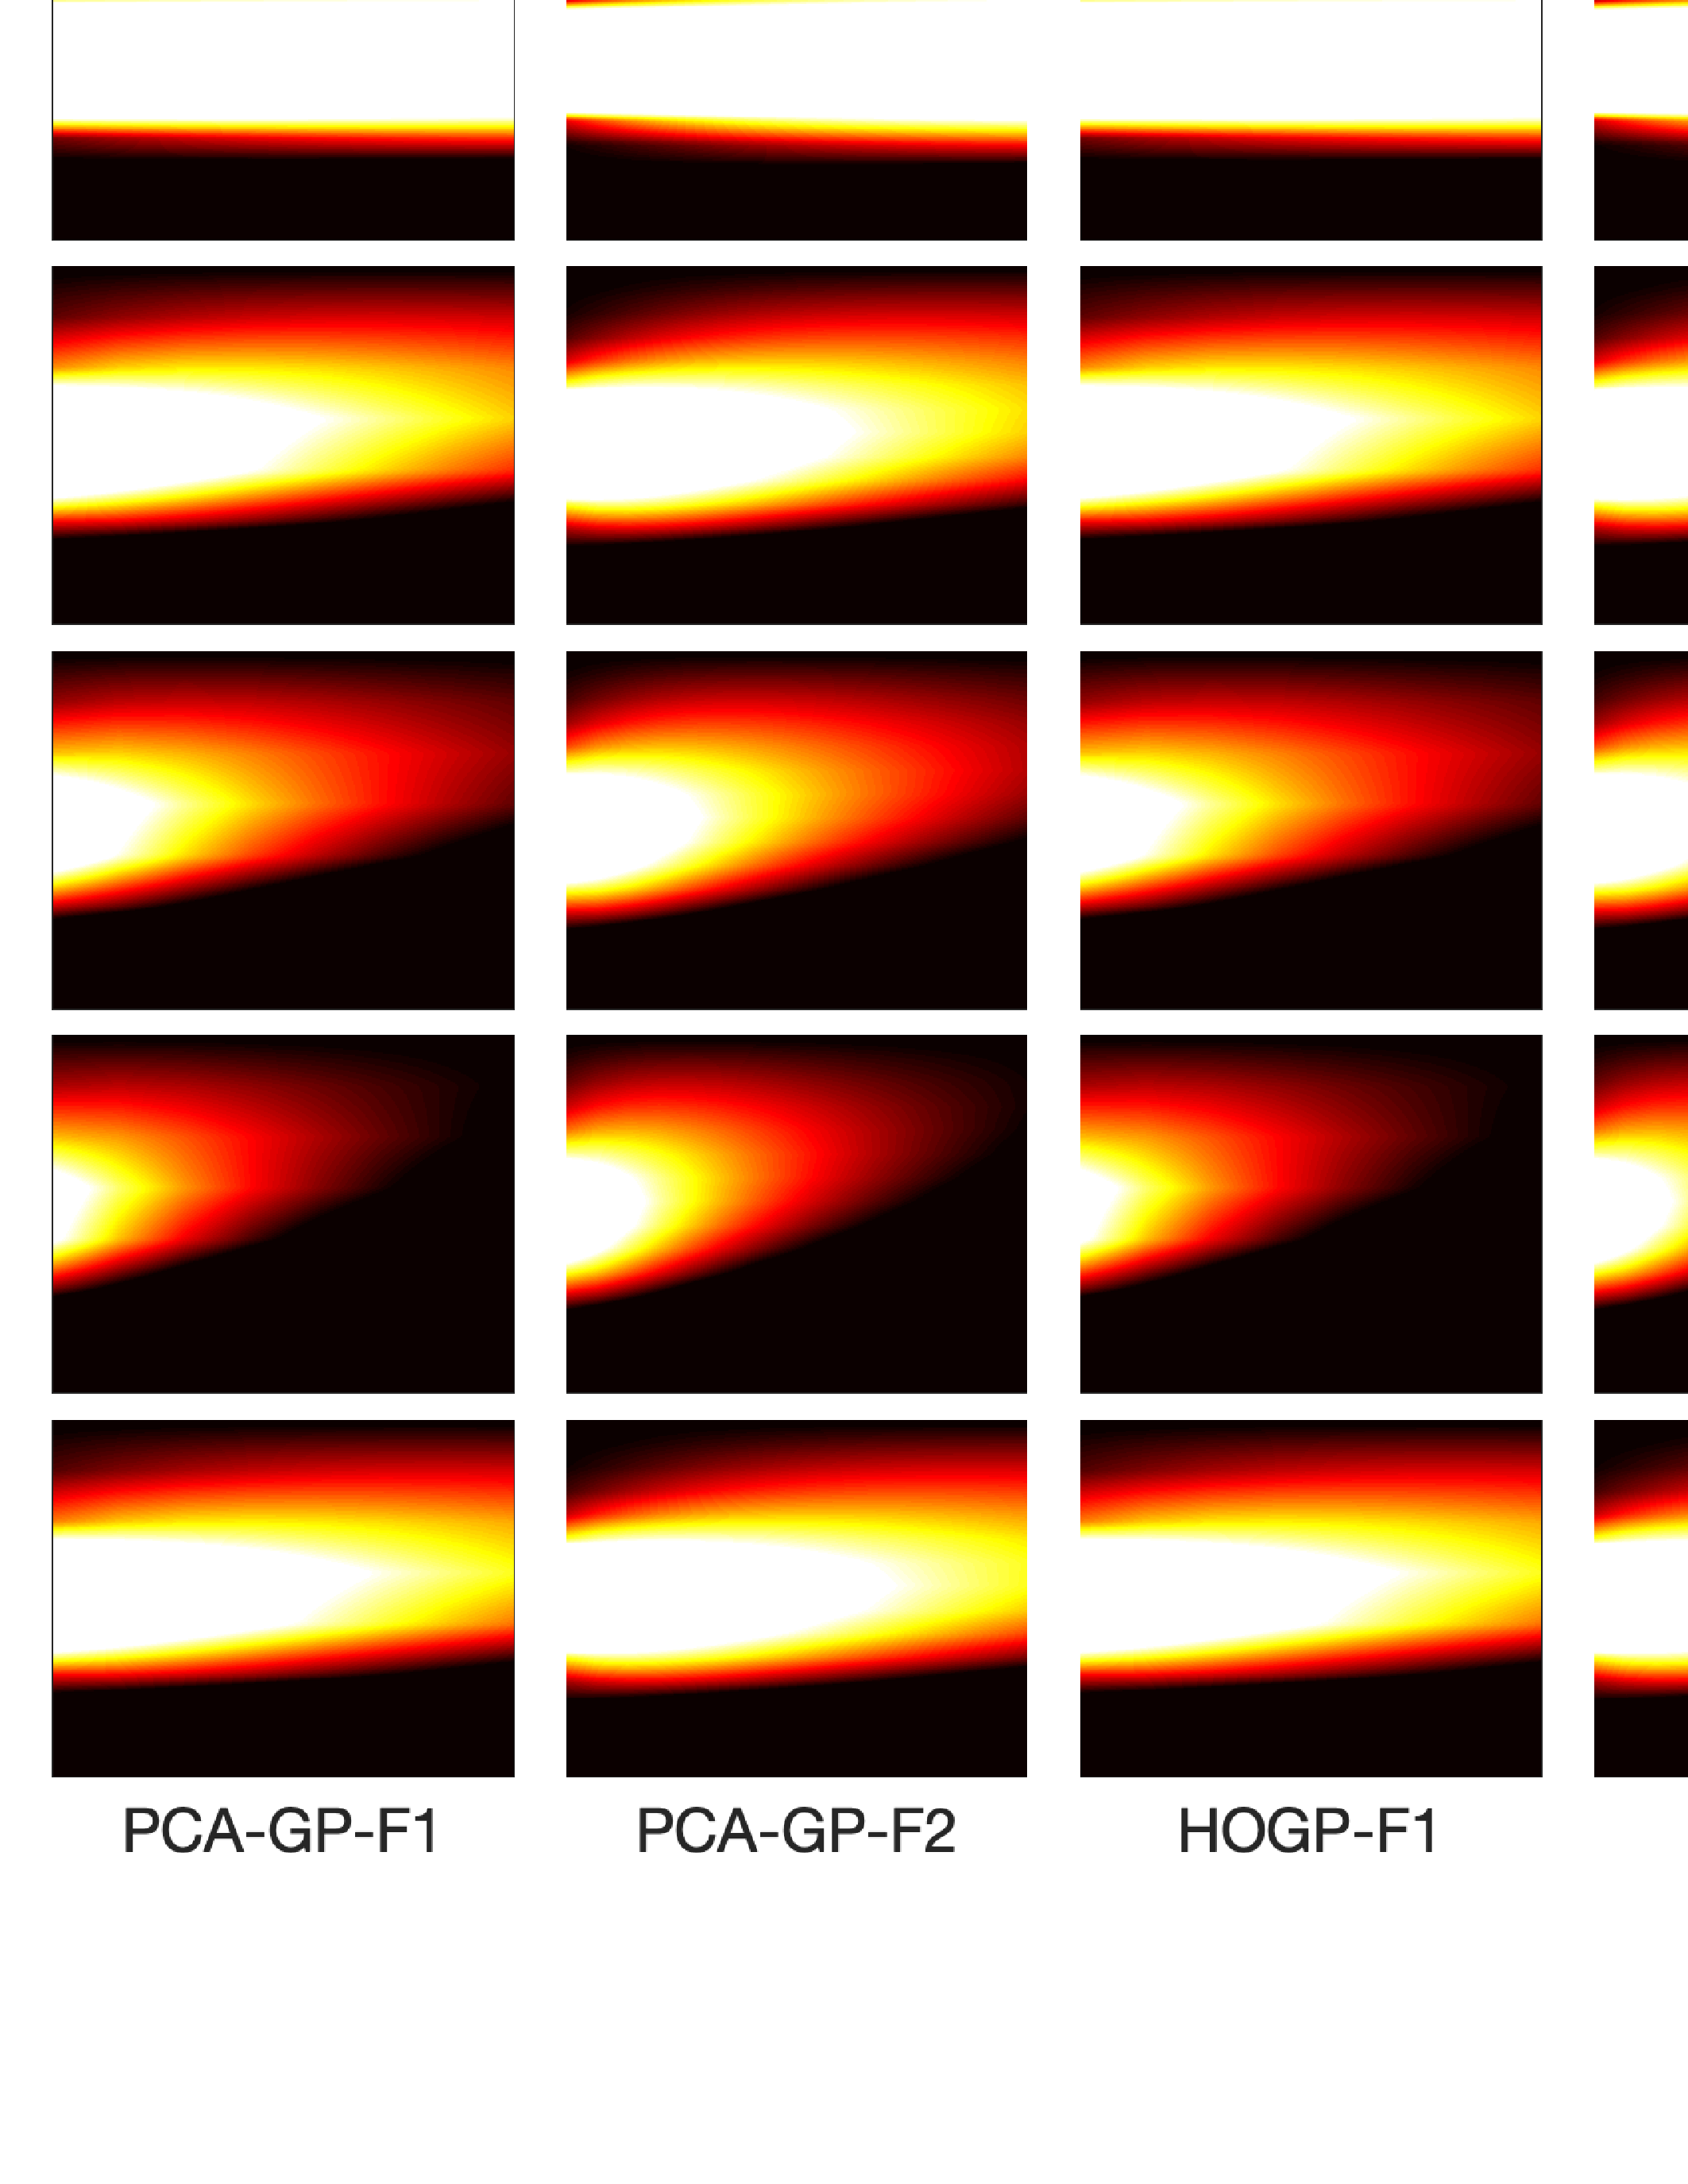}
	\caption{Actual predictive mean fields for Burger's equation using 256 fidelity-1 samples, 64 fidelity-2 samples, and $R=8$.}
	\label{ap:lv2_3}
\end{figure} 

%%%%%%%%%%%%%
\section{Actual Field Predictions for Three-fidelity Experiments}
\label{app:actual predictions lv3}
Six randomly selected actual predictive fields for Poisson's equation, the heat equation, and Burger's equation for all competing methods using 64 fidelity-1 samples, 16 fidelity-2 samples, 4 fidelity-3 samples, and $R=8$ is shown in Figs.~\ref{ap:lv3_1}, \ref{ap:lv3_2}, and \ref{ap:lv3_3}.

\begin{figure}[h]
	\centering
	\includegraphics[width=0.6\textwidth]{./fig_v2/instHeatMapBar.eps}
	\includegraphics[width=\textwidth]{./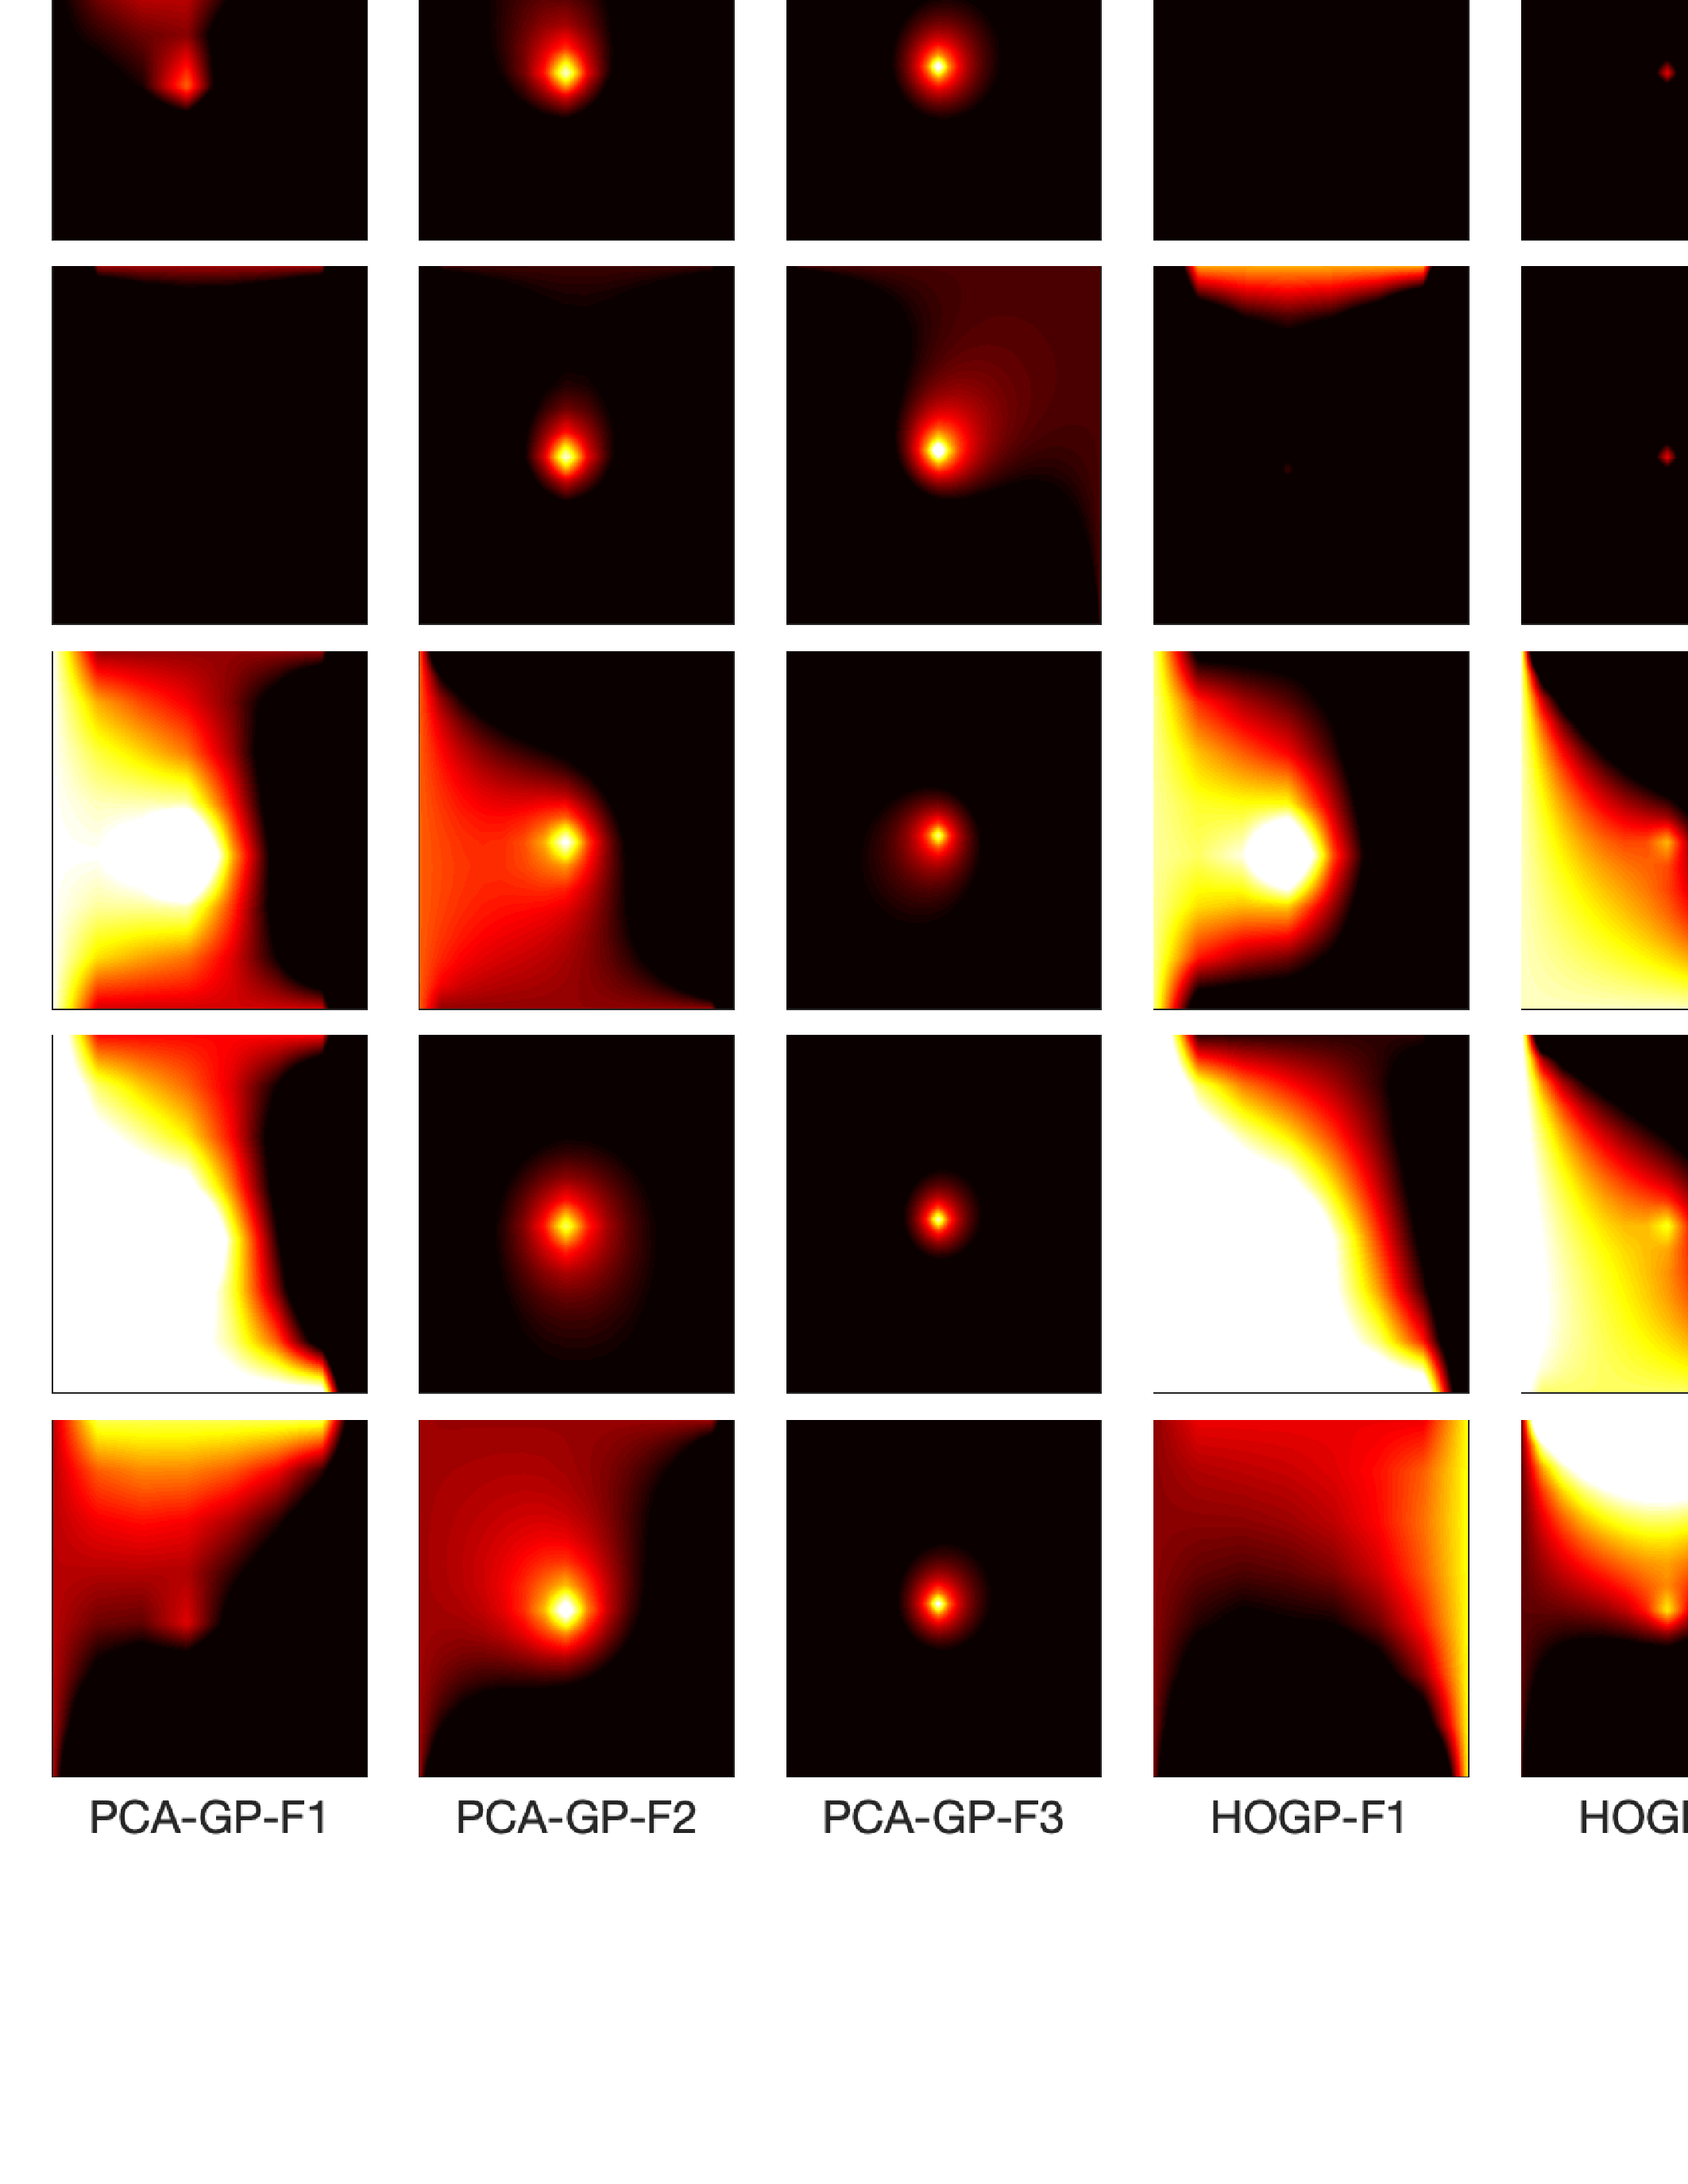}
	\caption{Actual predictive mean fields for Poisson's equation using 64 fidelity-1 samples, 16 fidelity-2 samples, 4 fidelity-3 samples, and $R=8$.}
	\label{ap:lv3_1}
\end{figure} 

\begin{figure}[h]
	\centering
	\includegraphics[width=0.6\textwidth]{./fig_v2/instHeatMapBar.eps}
	\includegraphics[width=\textwidth]{./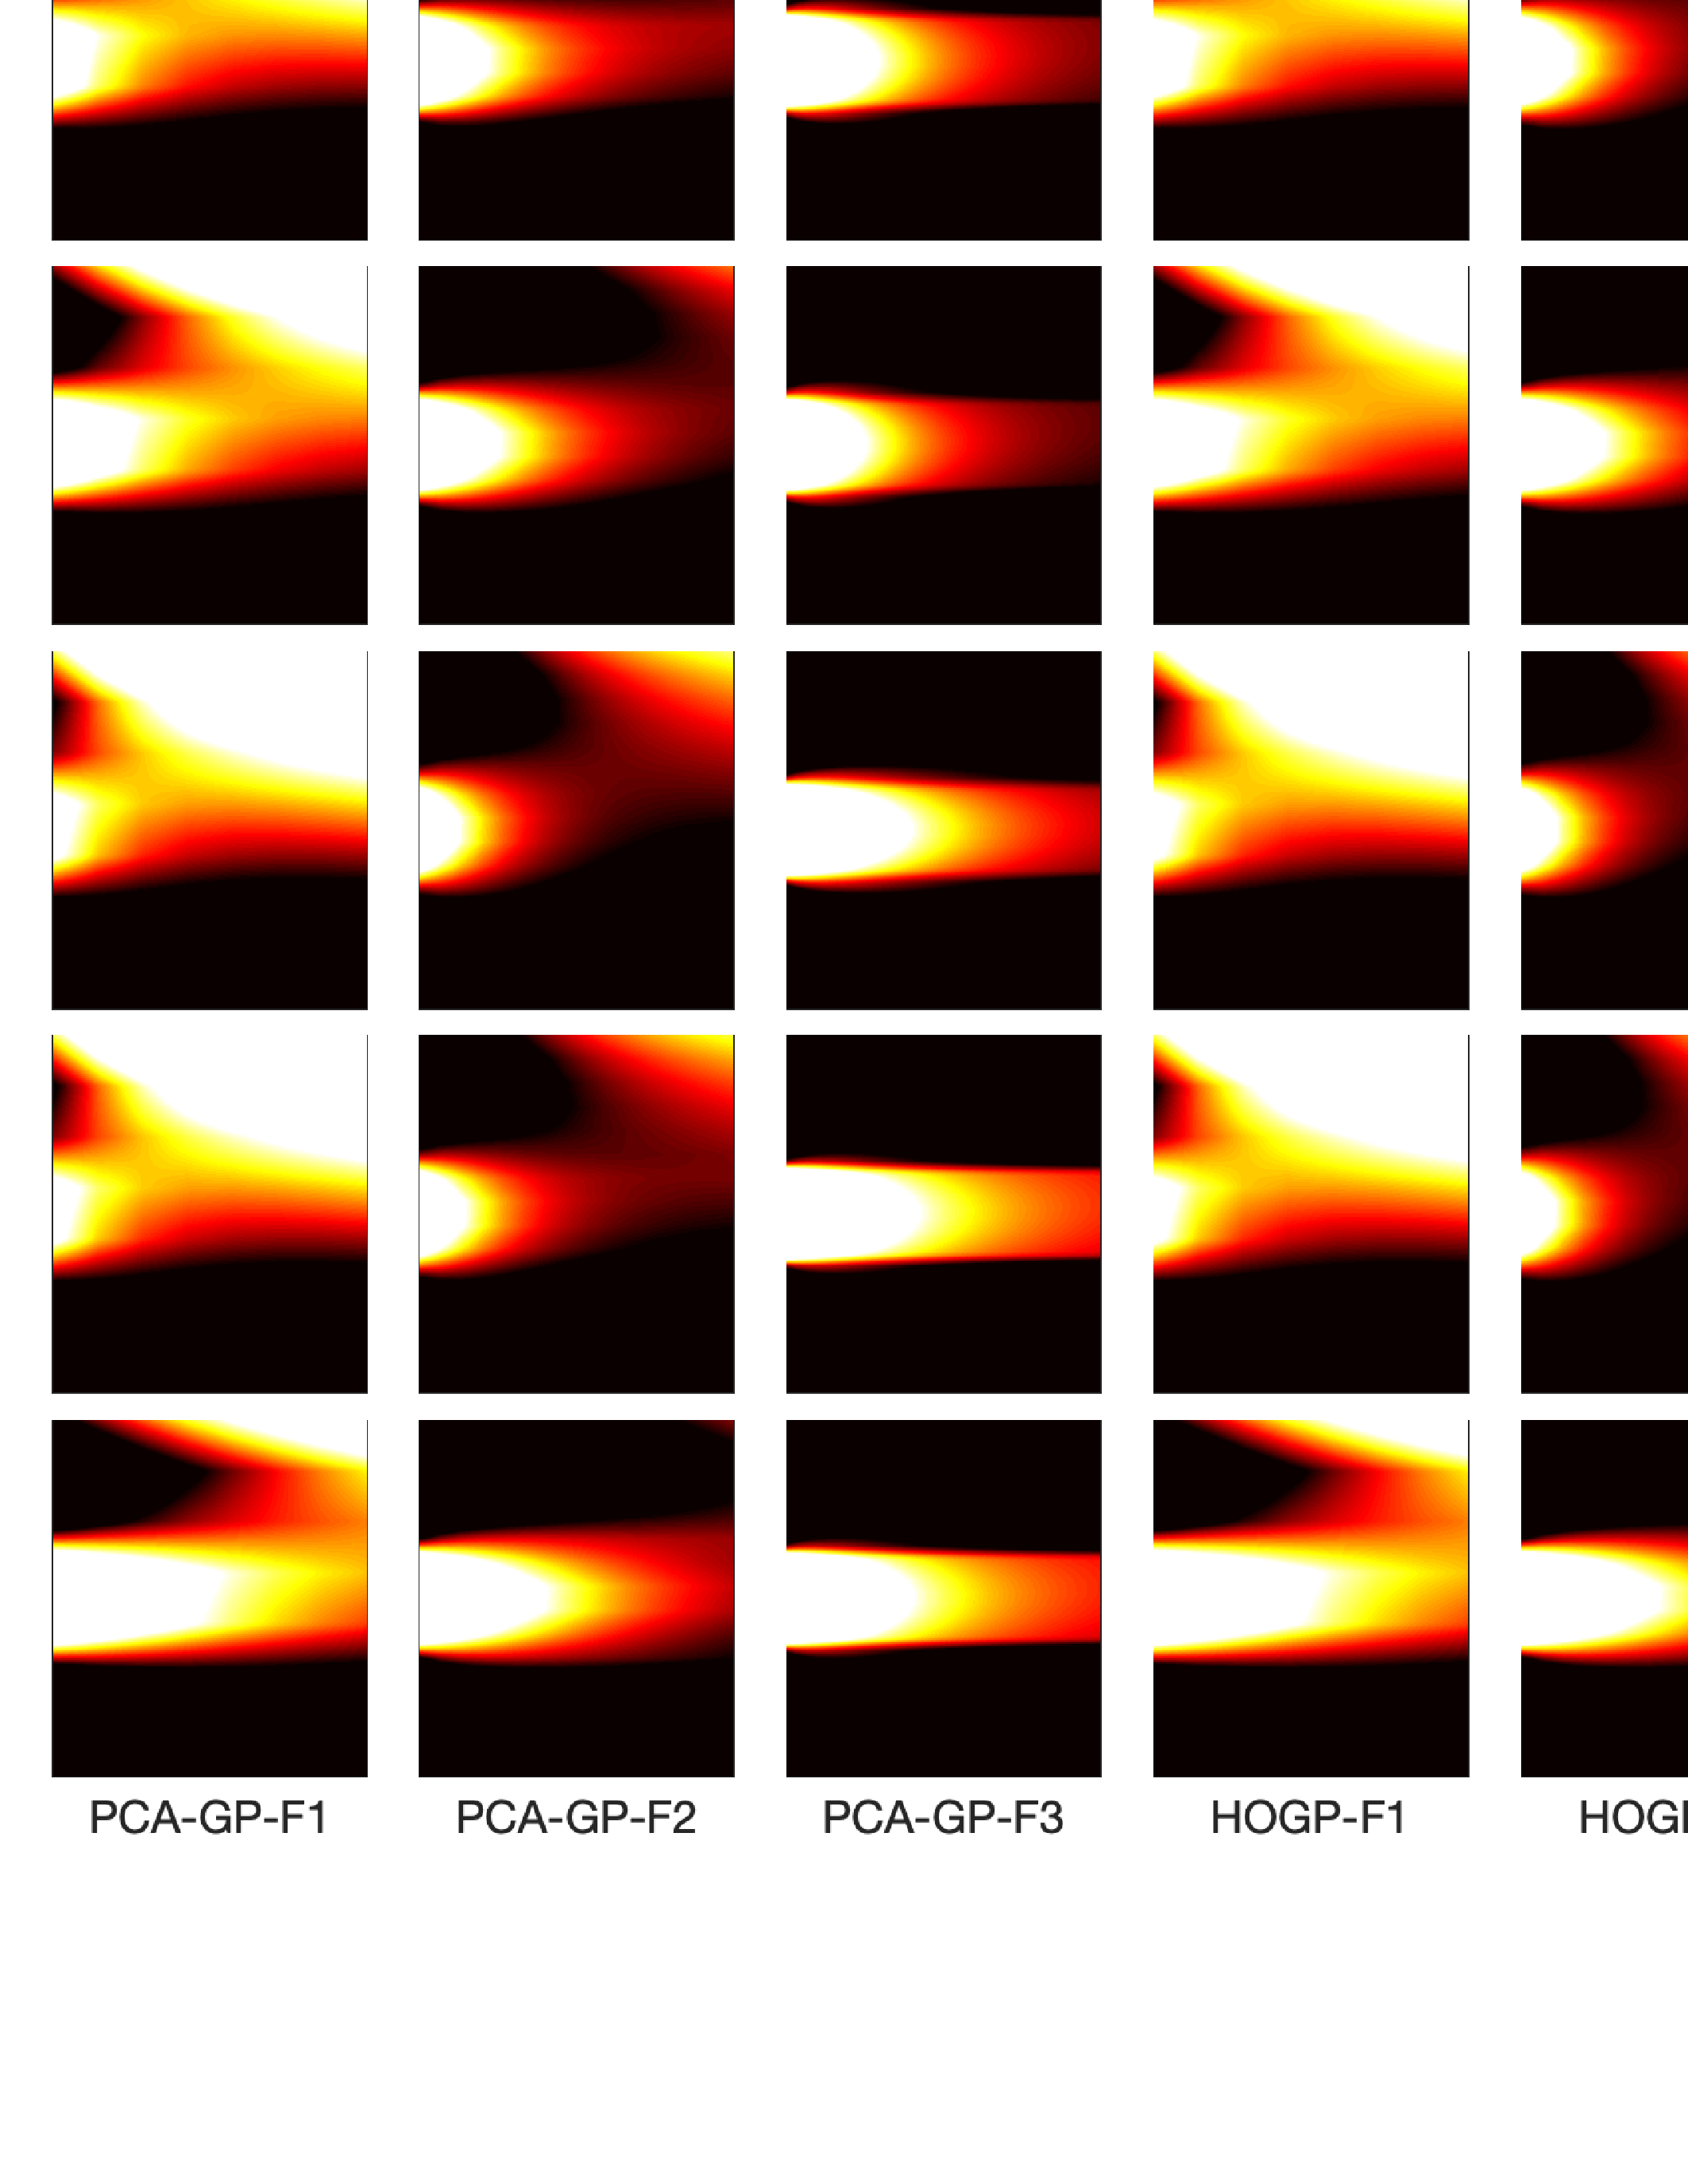}
	\caption{Actual predictive mean fields for heat equation using 64 fidelity-1 samples, 16 fidelity-2 samples, 4 fidelity-3 samples, and $R=8$.}
	\label{ap:lv3_2}
\end{figure}

\begin{figure}[h]
	\centering
	\includegraphics[width=0.6\textwidth]{./fig_v2/instHeatMapBar.eps}
	\includegraphics[width=\textwidth]{./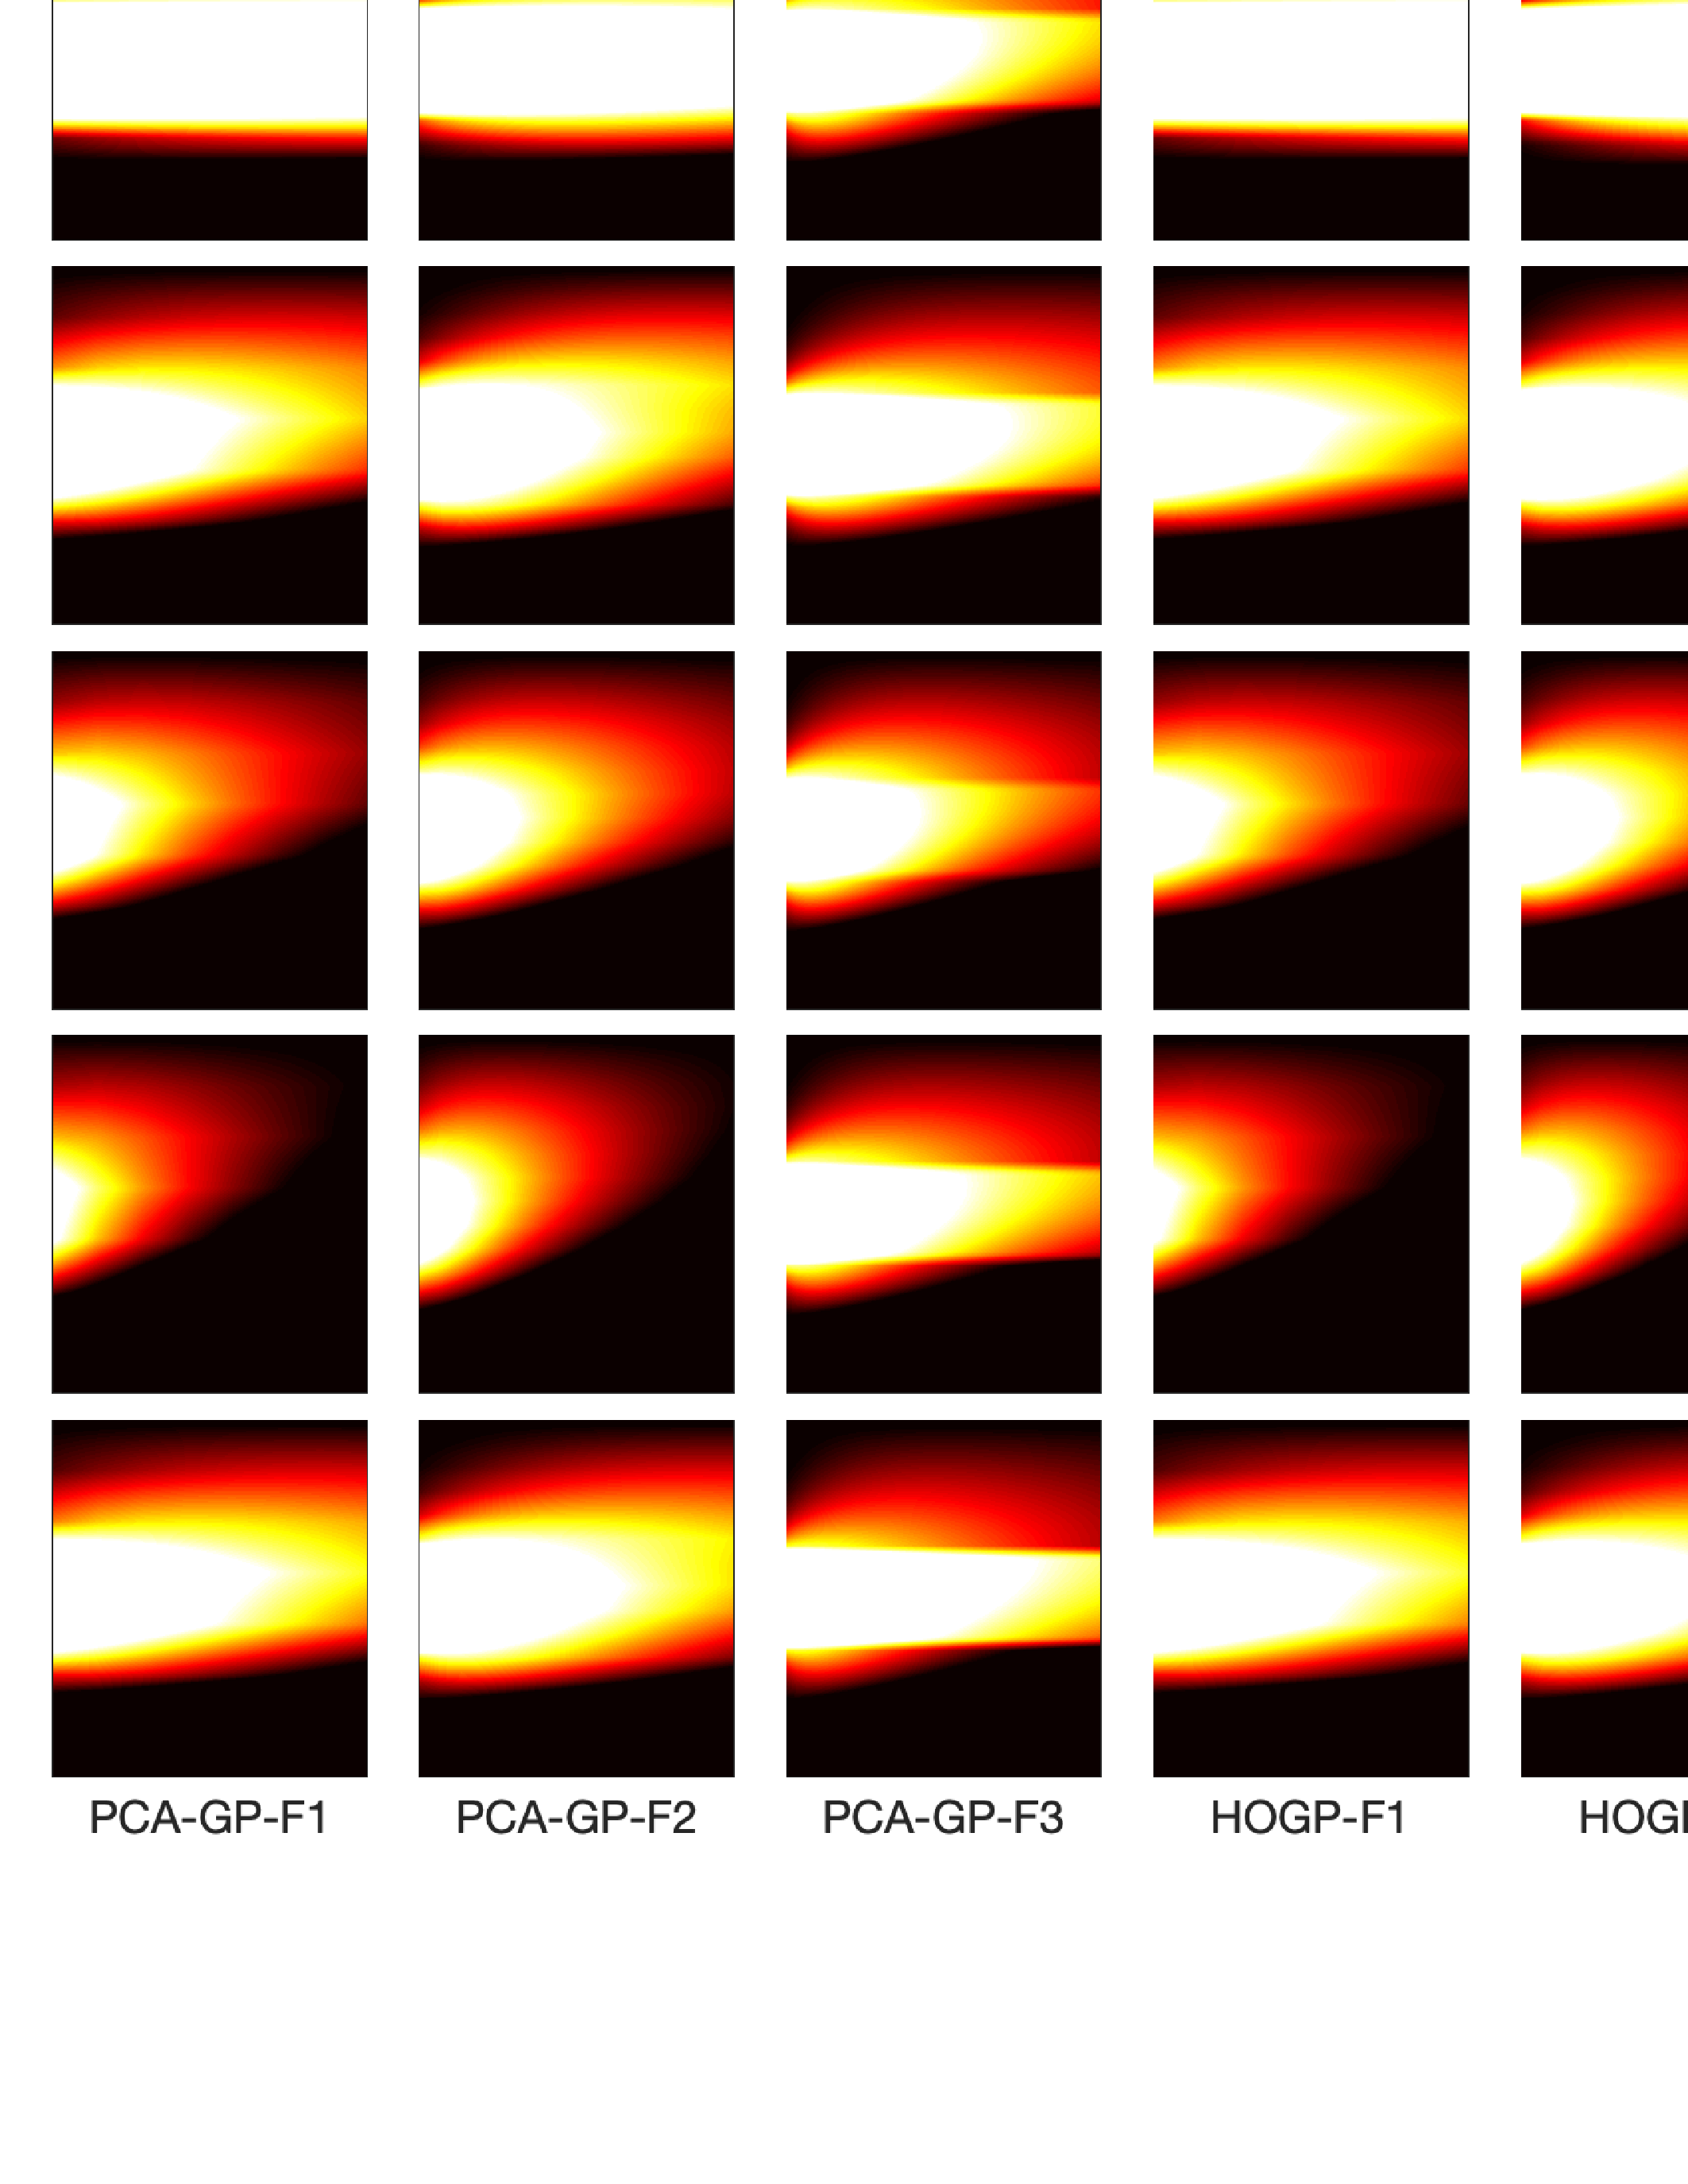}
	\caption{Actual predictive mean fields for Burger's equation using 64 fidelity-1 samples, 16 fidelity-2 samples, 4 fidelity-3 samples, and $R=8$.}
	\label{ap:lv3_3}
\end{figure} 

\end{appendices}
